# Supplementary material for: Implicit Neural Representations with Periodic Activation Functions
Source: arXiv:2006.09661 source file (2020-06-17)
Supplement: Supplementary file 1 [file supplement_applications_bvp.tex]

The Helmholtz and wave equations are second-order partial differential equations related to the physical modeling of diffusion and waves.  
They are closely related through a Fourier-transform relationship, with the Helmholtz equation given as  
\begin{equation}
    \underbrace{(\nabla^2 + m(\mathbf{x})w^2)}_{H(m)}\implicit(\mathbf{x}) = -f(\mathbf{x}).
    \label{eqn:helmholtz}
\end{equation}
Here, $f(\mathbf{x})$ represents a known source function, $\implicit(\mathbf{x})$ is the unknown wavefield, and the squared slowness $m(\mathbf{x}) = 1/c(\mathbf{x})^2$ is a function of the wave velocity $c(\mathbf{x})$.
In general, the solutions to the Helmholtz equation are complex-valued and require numerical solvers to compute.

\subsection{Helmholtz Perfectly Matched Layer Formulation}

To solve the Helmholtz equation uniquely over a finite domain, we use a perfectly matched layer formulation, which attenuates waves on the boundary of the domain.
Following Chen et al.~\cite{chen2013optimal} we rewrite the Helmholtz equation as  
\begin{equation}
    \frac{\partial}{\partial x_1} \left( \frac{e_{x_2}}{e_{x_1}} \frac{\partial \implicit(\mathbf{x})}{\partial x_1}\right)
    + \frac{\partial}{\partial x_2} \left( \frac{e_{x_1}}{e_{x_2}} \frac{\partial \implicit(\mathbf{x})}{\partial x_2}\right) + e_{x_1}e_{x_2}k^2 \implicit(\mathbf{x}) = -f(\mathbf{x})
    \label{eqn:pml}
\end{equation}
where $\mathbf{x} = (x_1, x_2) \in \Omega$, $e_{x_i} = 1 - j\frac{\sigma_{x_i}}{\omega}$, $k = \omega / c$, and 
\begin{align*}
\sigma_{x_i} = \begin{dcases}
a_0 \omega \left(\frac{l_{x_i}}{L_\text{PML}} \right)^2 & x_i \in \partial{\Omega} \\
a_0 \omega \left(\frac{l_{x_i}}{L_\text{PML}} \right)^2 & \text{else}
\end{dcases}.
\end{align*}
Here, $a_0$ controls the amount of wave attenuation (we use $a_0=5$), $l_{x_i}$ is the distance to the PML boundary along the $x_i$ axis, and $L_{\text{PML}}$ is the width of the PML. Note that the PML is applied only to the boundary of our domain $\partial{\Omega} = \{x \, | \, 0.5 < \lVert x \rVert_\infty < 1\}$ and that the equation is identical to the original Helmholtz equation elsewhere. To train \sinet{}, we optimize Eq.~\ref{eqn:pml} using the loss function described in the main paper with $\lambda(\mathbf{x}) = k = \text{batch size} / 5\times 10^3$. 

\subsection{Full-Waveform Inversion}
 
For known source positions and sparsely sampled wavefields, full-waveform inversion (FWI) can be used to jointly recover the wavefield and squared slowness over the entire domain.
Specifically, FWI involves solving the constrained partial differential equation  
\begin{equation}
    \argmin_{m, \Phi} \sum\limits_{1\le i\le N} \int_\Omega \lvert \Sha_r (\implicit_i(\mathbf{x}) - r_i(\mathbf{x})) \rvert^2\, d\mathbf{x}    \quad  \text{s.t.}\quad H(m)\,\implicit_i(\mathbf{x}) = -\gt_i(x) \quad 1\le i \le N, \,\forall \mathbf{x} \in \Omega,
    \label{eqn:fwi}
\end{equation}
where there are $N$ sources, $\Sha_r$ samples the wavefield at the receiver locations, and $r_i$ is the measured receiver data for the $i$th source.

We solve this equation with a principled method based on the alternating direction method of multipliers~\cite{boyd2011distributed,aghamiry2019improving}. 
To perform FWI with \sinet{}, we first pre-train the network to solve for the wavefields given a uniform velocity model.
This is consistent with the principled solver, which is initialized with a uniform velocity.
This pre-training process updates \sinet{} to minimize 
\begin{equation}
    \mathcal{L}_{\text{FWI, pretrain}} = \mathcal{L}_{\text{Helmholtz}}+ \lambda_{\text{slowness}} \mathcal{L}_{\text{slowness}}
\end{equation}
where the first term is as described in the main paper, and the last term is simply $\lVert m(\mathbf{x}) - m_0 \rVert_1$.
$m(\mathbf{x})$ is parameterized using a single output of \sinet{} and we use an initial squared slowness value of $m_0 = 1$ in our experiments.
The loss term $\mathcal{L}_\text{slowness}$ is calculated over all sampled locations $\mathbf{x}$ in each minibatch.
We also parameterize the multiple wavefields with additional \sinet{} outputs.
This is accommodated in the loss function by sampling all source locations at each optimization iteration and applying the loss function to the corresponding wavefield outputs.
Finally, we set $k = \text{batch size} / 10^4$ and $\lambda_{\text{slowness}} = \text{batch size}$.

After pre-training, we perform FWI using \sinet{} with a penalty method variation~\cite{van2013mitigating} of Eq.~\ref{eqn:fwi} as a loss function. This is formulated as 
\begin{equation}
    \mathcal{L}_{\text{FWI}} = \mathcal{L}_{\text{Helmholtz}} + \lambda_{\text{data}} \mathcal{L}_{\text{data}}
\end{equation}
where $\mathcal{L}_{\text{data}} = \sum\limits_i \lVert \implicit_i(\mathbf{x}) - r_i(x)\rVert_1 \Big\rvert_{x \in \Omega_r }$, and $\Omega_r$ is the set of receiver coordinates. In other words, we add a weighted loss term using the (PML) Helmholtz formulation on the receiver coordinates. Here we use the same values of $k$ and $\lambda_{\text{slowness}}$ as for pre-training.

\subsection{Helmholtz Implementation \& Reproducibility Details}
\paragraph{Data.}
The dataset consists of randomly sampled coordinates and a Gaussian source function, as described previously. For neural FWI, the data term of the loss function uses the sampled wavefield values from the output of the principled solver using the same source and receiver locations, but with access to the ground truth velocity.

\paragraph{Architecture.}
For all Helmholtz experiments, the \sinet{} architecture (and baselines) use 5 layers with a hidden layer size of 256.   

\paragraph{Hyperparameters.}
We set the loss function hyperparameters to the previously described values in order to make each component of the loss approximately equal during the beginning of training.
The Adam optimizer with a learning rate of $2\times 10^{-5}$ was used for all experiments. 

\paragraph{Runtime.}
The single-source Helmholtz experiments were trained for 50,000 iterations requiring approximately 3 hours (ReLU), 8 hours (tanh, \sinet{}), or 24 hours (RBF). For FWI, pretraining required 80,000 (22 hours) iterations in order to suitably fit the 5 wavefields with a single network, and then we performed full-waveform inversion for 10,000 iterations (5 hours) until the loss appeared to converge. We set the batch size to fill the GPU memory; generally, we found that large batch sizes ranging from 3000 to 13000 samples worked well.

\paragraph{Hardware.}
The experiments are conducted on a NVIDIA Quadro RTX 6000 GPU (24 GB of memory).

\subsection{Wave Equation Formulation}
The wave equation is given by 
\begin{equation}
    \frac{\partial \implicit}{\partial t} - c^2\frac{\partial \implicit}{\partial\mathbf{x}} = 0.
\end{equation}
Note that in contrast to the Helmholtz equation, the wave equation is dependent on time. 
Thus, we parameterize the real-valued wavefield as a function of two spatial dimensions and time: $\implicit(t, \mathbf{x})$. 
We are interested in solving an initial value problem with the following initial conditions 
\begin{align}
    &\frac{\partial \implicit(0, \mathbf{x})}{\partial t} = 0 \\
    &\implicit(0, \mathbf{x}) = f(\mathbf{x}).
\end{align}
In the case of the acoustic wave equation, the first condition states that the initial particle velocity is zero, and in the second condition, $f(\mathbf{x})$ is an initial pressure distribution.  

\subsection{Solving the Wave Equation}

We solve the wave equation by  parameterizing $\implicit(t, \mathbf{x})$ with \sinet{}.
Training is performed on randomly sampled points $\mathbf{x}$ within the domain $\Omega = \{\mathbf{x} \in \mathbb{R}^2 \, | \, \lVert \mathbf{x} \rVert_\infty < 1\}$.
The network is supervised using a loss function based on the wave equation:
\begin{equation}
    \mathcal{L}_{\text{wave}} = \int_\Omega \,\left\Vert \frac{\partial \implicit}{\partial t} - c^2\frac{\partial \implicit}{\partial\mathbf{x}} \right\Vert_1 + \lambda_{1}(\mathbf{x}) \left\Vert \frac{\partial \implicit}{\partial t} \right\Vert_1 + \lambda_{2}(\mathbf{x}) \left\Vert \implicit - f(\mathbf{x}) \right\Vert_1\,d\mathbf{x}.
\end{equation}
Here, $\lambda_1$ and $\lambda_2$ are hyperparameters, and are non-zero only for $t=0$. To train the network, we sample values of $\mathbf{x}$ uniformly from $\Omega$ and slowly increase the value of $t$ linearly as training progresses, starting from zero. This allows the initial condition to slowly propagate to increasing time values. We set $\lambda_1=\text{batch size}/100$ and $\lambda_2 = \text{batch size}/10$ and let $c=1$. 

Results are shown in Fig.~\ref{fig:wave} for solving the wave equation with $f(\mathbf{x})$ equal to a Gaussian centered at the origin with a variance of $5\times 10^{-4}$. We also compare to a baseline network with tanh activations (similar to recent work on neural PDE solvers~\cite{raissi2019physics}), and additional visualizations are shown in the video. \sinet{} achieves a solution that is close to that of a principled solver~\cite{treeby2010k} while the tanh network fails to converge to a meaningful result. 

\subsection{Wave Equation Implementation \& Reproducibility Details} 
\paragraph{Data.}
The dataset is composed of randomly sampled coordinates 3D coordinates as described previously. We use a Gaussian source function to approximate a point source, and clip the support to values greater than 1e-5. During training, we scale the maximum value of the Gaussian to 0.02, which we find improves convergence. 

\paragraph{Architecture.}
To fit over the 3 dimensions of the wave equation, we increase the size of the architecture, still using 5 layers, but with a hidden layer size of 512. 

\paragraph{Hyperparameters.}
 The loss function hyperparameters are set so that each component of the loss is approximately equal as training progresses. We grow the interval of $t$ from which training coordinates are sampled linearly over 100,000  iterations (roughly 25 hours) from 0.0 to 0.4, which we find allows a sufficient number of iterations for the network to fit the wave function as it expands. For all wave equation experiments, we used the ADAM optimizer and a learning rate of $2 \times 10^{-5}$. A batch size of 115,000 is used, which fills the GPU memory.

 \paragraph{Hardware.} The experiments are conducted on a NVIDIA Quadro RTX 6000 GPU (24 GB of memory).

\begin{figure}
    \centering
    \includegraphics[]{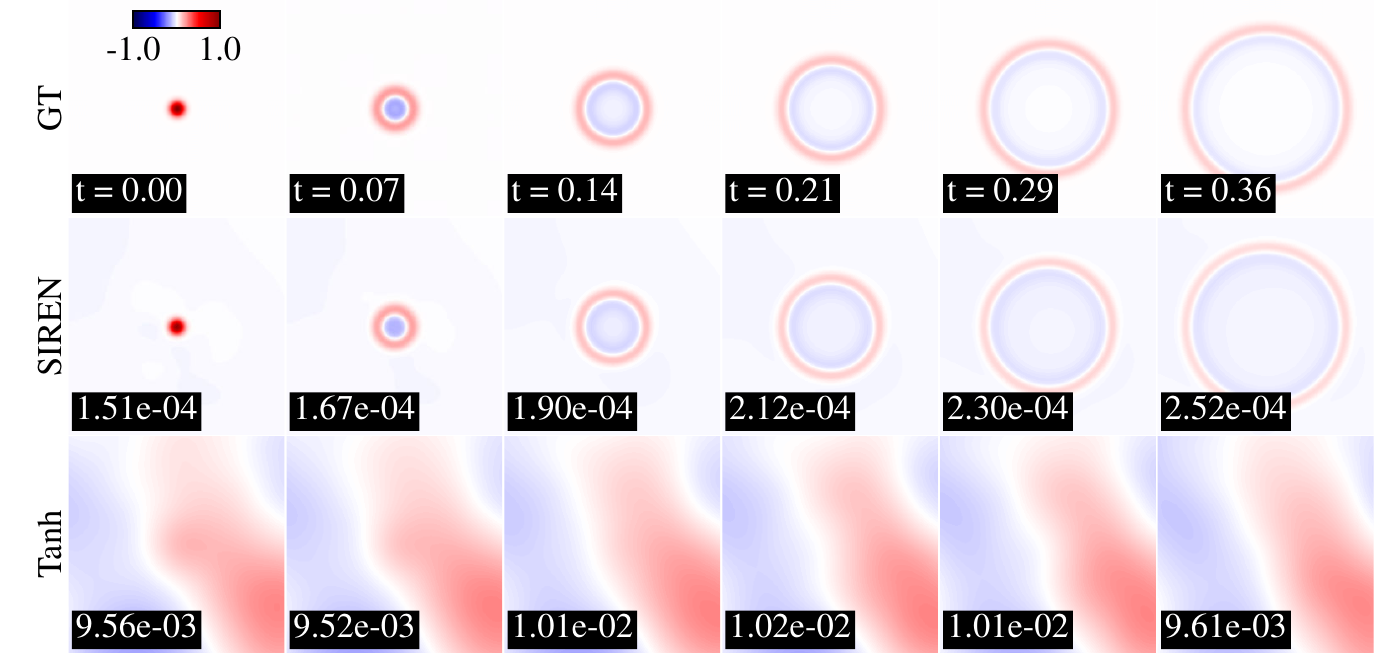}
    \caption{Solving the wave equation initial value problem. For an initial condition corresponding to a Gaussian pulse, \sinet{} recovers a wavefield that corresponds closely to a ground truth wavefield computed using a principled wave solver~\cite{treeby2010k}. A similar network using tanh activations fails to converge to a good solution. MSE values are shown for each frame, where the time value is indicated in the top row.}
    \label{fig:wave}
\end{figure}
