# Supplementary material for: Implicit Neural Representations with Periodic Activation Functions
Source: arXiv:2006.09661 source file (2020-06-17)
Supplement: Supplementary file 2 [file supplement_applications_imaging.tex]

\subsection{Formulation}
As shown previously, one example of signal that \sinet{}s can be used to represent are natural images. A continuous representation of natural images with a \sinet{} introduces a new way to approach image processing tasks and inverse problems. Consider a mapping from continuous implicit image representation $\implicit(x,y)$ to discrete image $\lowresimg$
\begin{equation}
\lowresimg = \samplingop \left( \downsamplingkernel * \implicit_{\implicitparams} \left( x, y \right) \right),
\label{eq:continuous to discrete}
\end{equation}
where $\samplingop$ is the sampling sampling operator, $\downsamplingkernel$ is a downsampling filter kernel, and $\implicit(x,y)$ is the continuous implicit image representation defined by its parameters $\implicitparams$. Using this relationship, we can fit a continuous \sinet{} representation given a discrete natural image $\lowresimg$ by supervising on the sampled discrete image.

Many image processing problems can be solved by formulating an optimization problem which minimizes data fidelity with partial or noisy measurements of $\lowresimg$ and some prior over natural images. In our case, our prior is over the space of \sinet{} representations of natural images. This takes the form:
\begin{equation}
\underset{\left\{ \implicitparams \right\}}{\textrm{minimize}} \,\, \loss \left( \samplingop \left( \downsamplingkernel * \implicit_{\implicitparams} \left( x, y \right) \right), \lowresimg \right) + \lambda \regularizer \left( \implicit_{\implicitparams} \left( x, y \right) \right),
\label{eq:objectivefun}
\end{equation}
where $\regularizer$ is a regularization function defined on the continuous function, and $\lambda$ is the weight of the regularizer.
\begin{figure}
	\centering
	\includegraphics[width=0.9\linewidth]{supplemental_figures/representation_figure_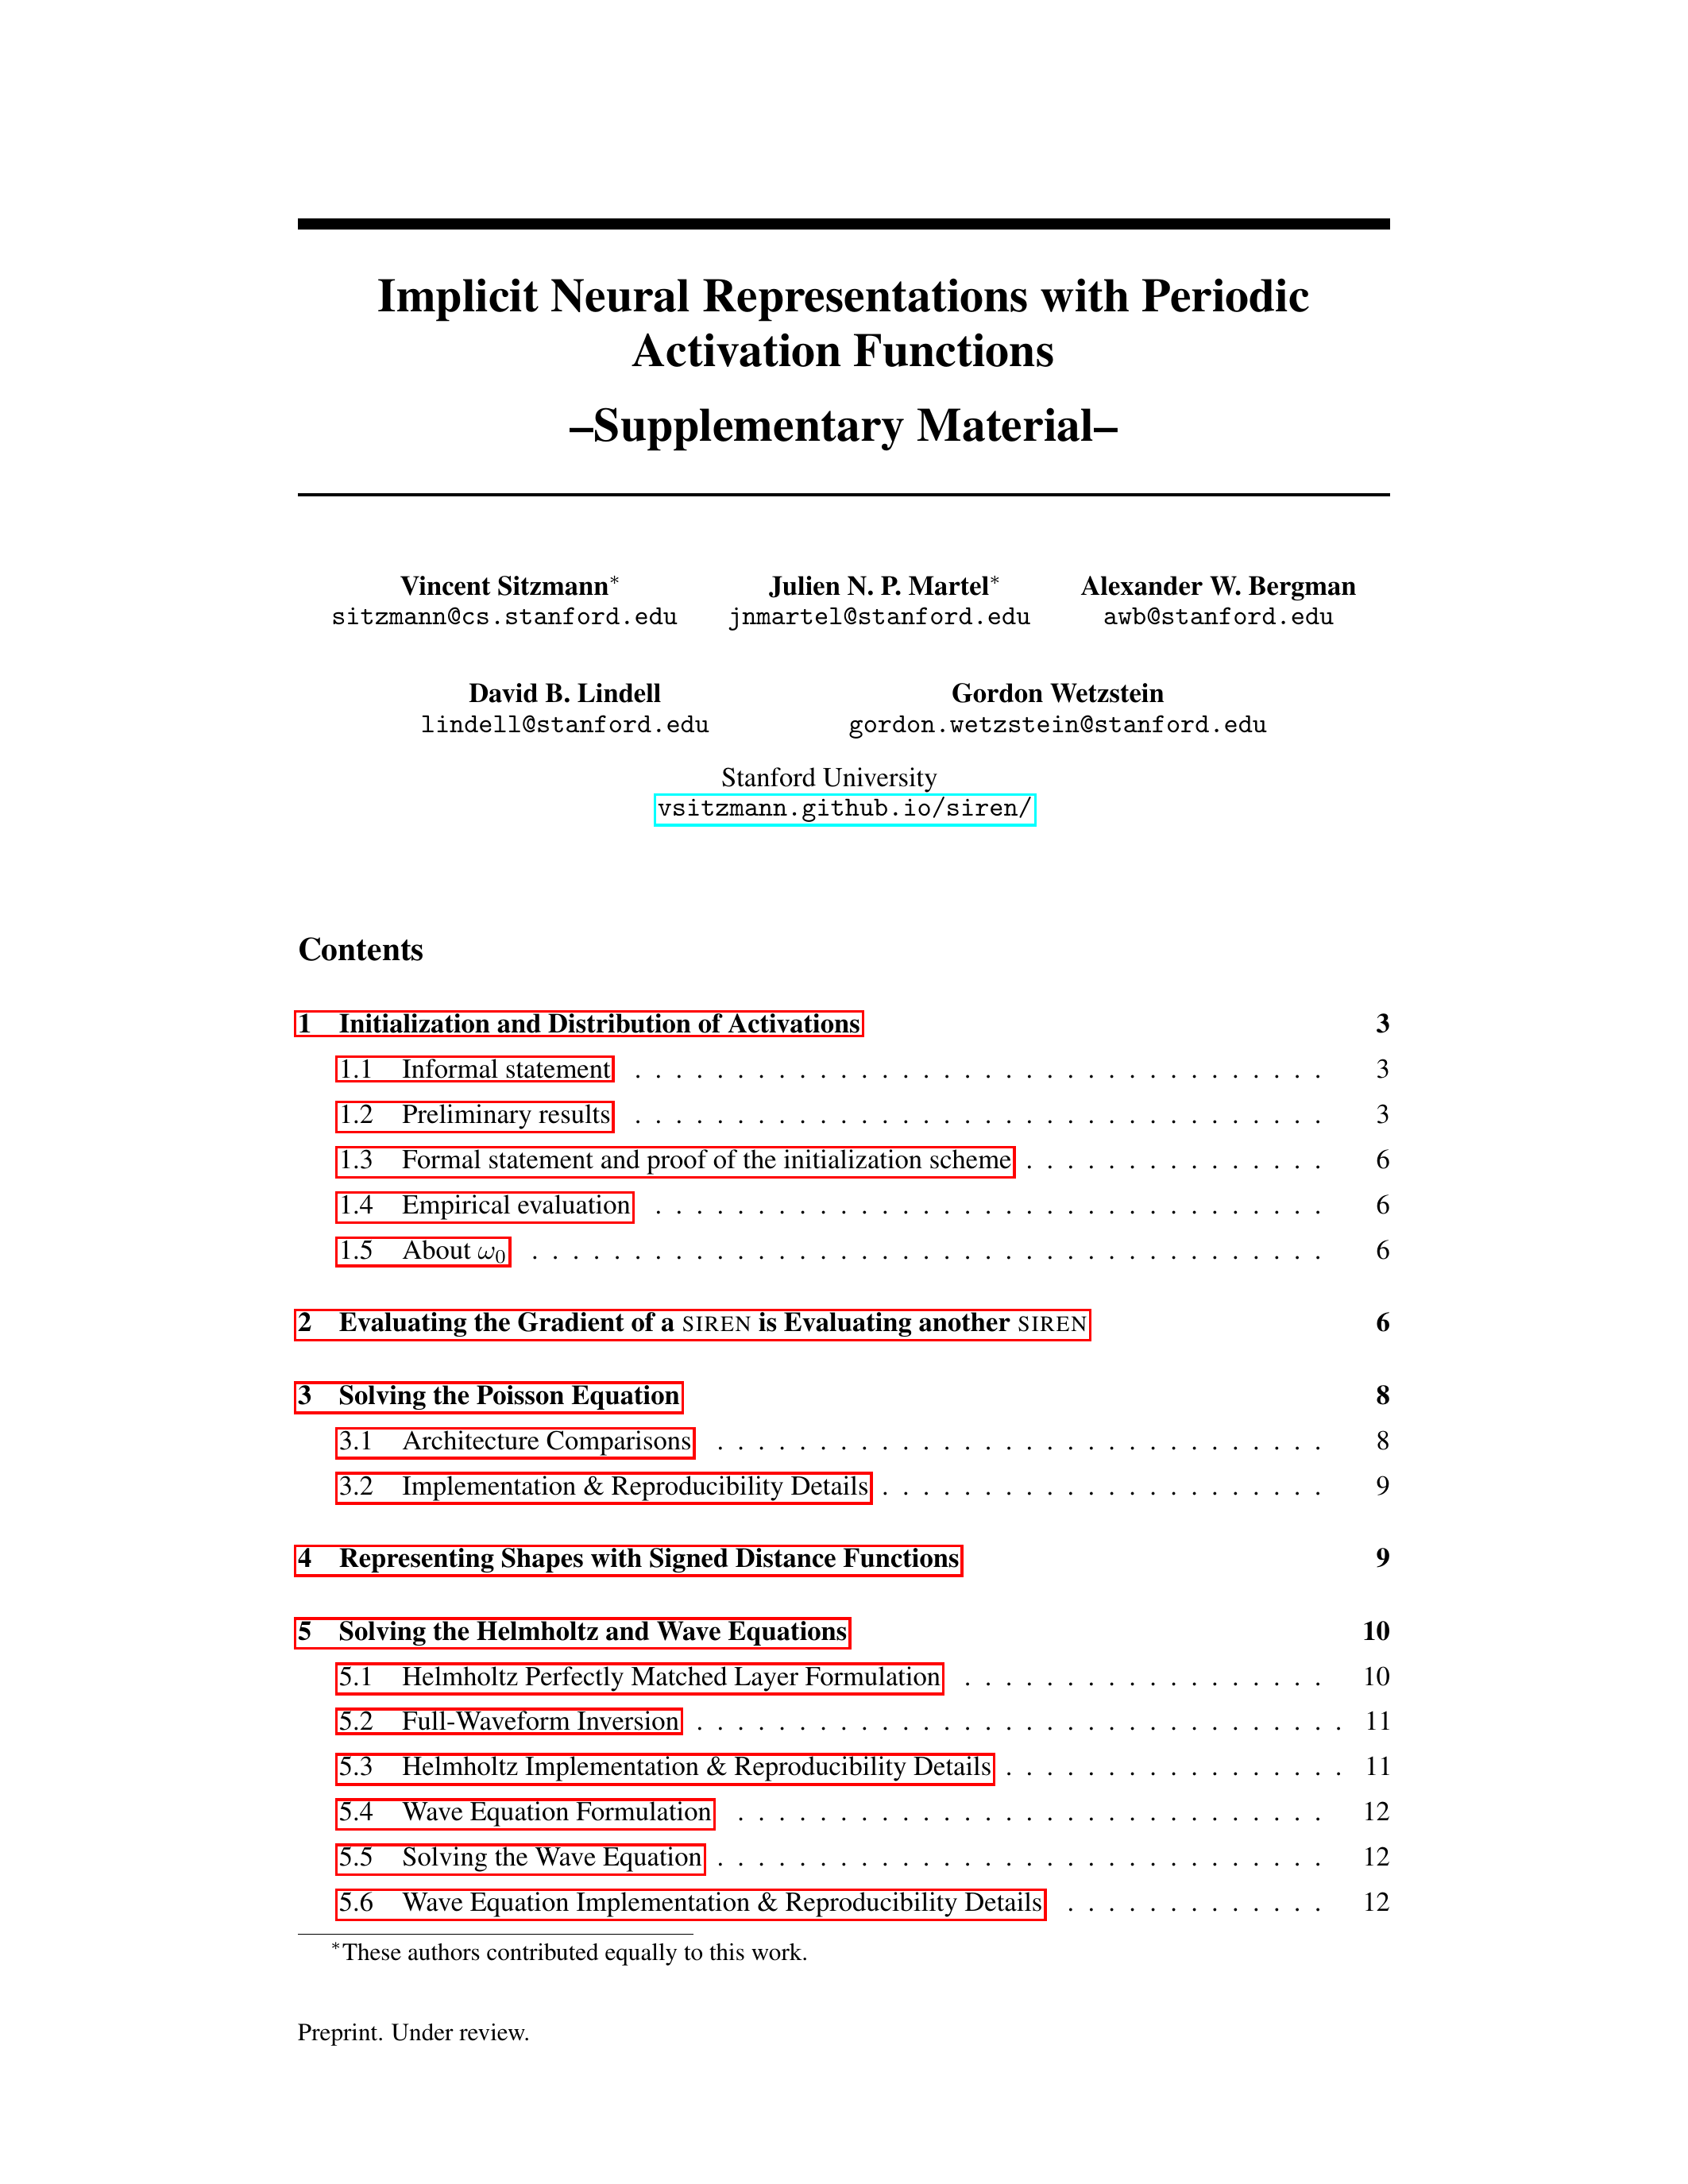}
	\caption{Comparison of different implicit network architectures fitting a ground truth image (top left). The representation is only supervised on the target image but we also show first- and second-order derivatives of the function fit in rows~2 and~3, respectively. We compare with architectures implemented using Softplus, ELU, SELU, and ReLU P.E. (L=4) on the cameraman image. The value of L dictates the number of positional encodings concatenated for each input coordinate, and a choice of $L=4$ was made for images in \cite{mildenhall2020nerf}.}
	\label{fig:imagefit_supplement}
\end{figure}

\subsection{Image Fitting.} 
As previously shown, the most simple representation task involves simply fitting an implicit neural representation $\implicit:\mathbb{R}^2 \mapsto \mathbb{R}^3, \coords \to \implicit(\coords)$ to an image. Simply fitting the image proves to be challenging for many architectures, and fitting higher-order derivatives is only possible using \sinet{}s. In addition to the comparisons with ReLU, tanh, ReLU P.E., and ReLU with RBF input layer shown in the paper, we show a qualitative comparison with additional neural network architectures in Fig.~\ref{fig:imagefit_supplement}.

\subsection{Image Inpainting}
Traditional approaches to the single image inpainting task have either focused on diffusion-based~\cite{Bertalmio2000Inpainting, Ballester2001Inapinting, Bertalmio2001cvpr} or patch based reconstruction~\cite{barnes2009patchmatch, kwatra2005patch, efros2001quilting}. 
With the advent of deep learning, a slew of new methods have taken advantage of large amounts of data to learn complex statistics of natural images used in reconstruction problems. These inpainting methods are based on convolutional neural networks (CNNs)~\cite{Liu2018ECCV,ren2019structureflow} and generative adversarial networks (GANs)~\cite{IizukaSIGGRAPH2017, Yu2019ICCV, Liu_2019_CSA, ma2019regionwise}. 
Additionally, neural network architectures for image recovery like CNNs have been shown to themselves act as a prior~\cite{ulyanov2017deep} for natural images, allowing for solving inverse problems without the use of training data.

We show the capability of \sinet{}s to solve inverse problems through the example of single image inpainting. By fitting a \sinet{} to an image and enforcing a prior on the representation, we can solve a single image reconstruction problem. 
Examples of single image inpainting with and without priors are shown in Fig.~\ref{fig:single_inpainting}, where we compare performance on texture images versus Deep Image Prior~\cite{ulyanov2017deep}, Navier-Stokes, Fluid Dynamics Image Inpainting~\cite{Bertalmio2001cvpr} (Diffusion), and \sinet{}s with no prior, total variation prior (TV), and Frobenius norm of Hessian~\cite{lysaker2003frobhessian, lysaker2006frobhessian} priors (FH) respectively. In Tab.~\ref{tab:inpainting}, we describe our quantitative results with mean and standard deviation over many independent runs.
These results show that \sinet{} representations can be used to achieve comparable performance to other baseline methods for image inverse problems.

Note that this formulation of loss function can be equivalently formulated in a continuous partial differential equation, and depending on choice of prior, a diffusion based update rule can be derived. For more details on this, see the Rudin–Osher–Fatemi model in image processing~\cite{gilles2010PDEbook, aubert2005pdeimg, getreuer2012PDE}.

\subsection{Implementation \& Reproducibility Details}

\paragraph{Data.} The experiments were run on texture images, including the art image of resolution $513\times513$ and tiles image of resolution $355\times533\times3$. These images will be made publicly available with our code. The sampling mask is generated randomly, with an average of 10\% of pixels being sampled. We will make the example mask for which these results were generated publicly available with our code. As in all other applications, the image coordinates $\mathbf{x}\in\mathbb{R}^2$ are normalized to be in the range of $[-1,1]^2$. For evaluation, images are scaled in the range of $[0,1]$ and larger values are clipped.

\paragraph{Architectures.} For the single image inpainting task with \sinet{}s, we use a 5-layer MLP. For single image fitting on the cameraman image, we use 5-layer MLPs for all activation functions. For the RBF-Input and ReLU P.E. models, we add an additional first layer with $256$ activations (in the case of RBF-Input) or positional encoding concatenation with positional encoding sinusoid frequencies of $2^i\pi$ for $0\leq i<L=7$ (in the case of ReLU P.E.).
\begin{figure}[t!]
	\includegraphics[width=\textwidth]{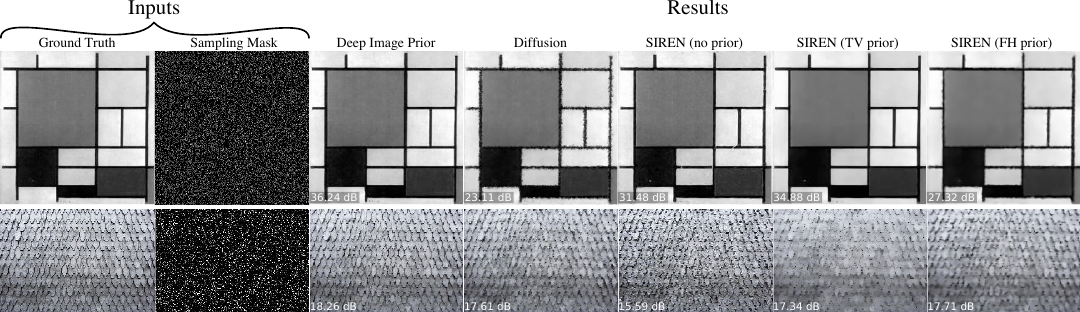}
	\caption{Comparison of various methods and priors on the single image inpainting task. We sample 10\% of pixels from the ground truth image for training, learning a representation which can inpaint the missing values. Note that for the image in the first row, where the TV prior is known to be accurate, including the TV prior improves inpainting performance.}
	\label{fig:single_inpainting}
\end{figure}

\paragraph{Loss Functions.} In order to evaluate a prior loss, we must enforce some condition on the higher-order derivatives of the \sinet{}. This is done by sampling $N$ random points $\mathbf{x}_i\in [-1,1]^2$, and enforcing the prior on these points. We sample half as many points for the prior as there are pixels in the image. In the case of TV regularization, this consists of a L1 norm on the gradient 
\begin{equation}
	\gamma_{\text{TV}} = \frac{1}{N}\sum_{i=1}^{N}|\nabla \implicit_{\implicitparams}(\mathbf{x}_i)|,
\end{equation} 
while in the case of FH regularization, this consists of L1 norm on all sampled points' Frobenius norm of their Hessian matrix
\begin{equation}
\gamma_{\text{FH}} = \frac{1}{N}\sum_{i=1}^{N}\|\text{Hess}(\implicit_{\implicitparams}(\mathbf{x}_i))\|_F.
\end{equation} 
The prior loss is weighted with a regularization weight $\lambda$, and combined with the MSE loss on the reconstructed sampled and blurred image points,
\begin{equation}
\loss_{\text{img}} = \|  \samplingop \left( \downsamplingkernel * \implicit_{\implicitparams} \left( x, y \right) \right) - \lowresimg \|^2.
\end{equation} 
%.

\paragraph{Downsampling Kernel Implementation.}
Sampling images from a continuous function requires convolution with a downsampling kernel to blur high frequencies and prevent aliasing. Since we cannot perform a continuous convolution on a \sinet{} we must instead approximate with Monte Carlo sampling of the \sinet{} to approximate fitting the blurred function. Consider the 2D image signal where $\mathbf{x}=(x,y)$:
\begin{equation}
\left( h*\implicit \right)\left(x,y\right) = \int_{x'}\int_{y'}\implicit\left( x',y' \right) \cdot h(x-x', y-y') dy'dx' \approx \frac{1}{N}\sum_{i=1}^{N} \implicit(x+x_i,y+y_i)
\end{equation}
where $x_i, y_i$ are sampled from the kernel $h$ as a normalized probability density function. For example, a bilinear downsampling kernel is given by $h(x,y)=\max(0,1-|x|)\max(0,1-|y|)$. Thus, we sample $x_i,y_i$ from a  probability density function of $p(x_i,y_i)=\frac{1}{2}\max(0,1-|x|)\max(0,1-|y|)$. 
In our implementation, we found that not using a downsampling kernel resulted in equivalent performance on the inpainting and image fitting task. However, it may be necessary in cases where we aim to reconstruct our image at multiple resolutions (i.e. superresolution). We only sample one blurred point, i.e. $N=1$, per iteration and train for many iterations. This is done for computational efficiency, as otherwise it is necessary to backpropagate the loss from all sampled coordinates.

\paragraph{Hyperparameters.} For the image fitting experiment, we train all architectures using the Adam optimizer and a learning rate of $1\times10^{-4}$. Hyperparameters were not rigorously optimized and were found by random experimentation in the range of $[1\times 10^{-6}, 1\times 10^{-4}]$. We train for 15,000 iterations, fitting all pixel values at each iteration.

For the image inpainting experiments, we use the published and OpenCV~\cite{opencv_library} implementations for the baseline methods, and use an Adam optimizer with a learning rate of $5\times 10^{-5}$ for all \sinet{} methods. We train for 5,000 iterations, fitting all pixel values at each iteration. For the TV prior, we use a regularization weight of $\lambda=1\times10^{-4}$, while for the FH prior, we use a regularization weight of $\lambda=1\times10^{-6}$.

\paragraph{Central Tendencies of Metrics.}
In Tab.~\ref{tab:inpainting}, we show the central tendencies (mean and standard deviation) of the quantitative PSNR scores obtained on the image inpainting experiment. Inpainting with \sinet{}s is highly stable and not sensitive to the specific pixel mask sampled. 

\begin{table}
	\vspace{-.3cm}
	\caption{Mean and standard deviation of the PSNR of the tiles texture and art texture images for \sinet{}s with various priors. The statistics are computed over 10 independent runs.}
	\label{tab:inpainting}
	\centering
	\begin{tabular}{l|cc|cc|cc}
		\toprule
		 & No Prior & No Prior & TV Prior & TV Prior & FH Prior & FH Prior \\
		Image & Mean PSNR & Std. PSNR & Mean PSNR & Std. PSNR & Mean PSNR & Std. PSNR \\
		\midrule
		Tiles & 15.45 & 0.180 & 17.40 & 0.036 & 17.68 & 0.051 \\
		Art & 32.41 & 0.283 & 34.44 & 0.222 & 27.18 & 0.116 \\
		\bottomrule
	\end{tabular}
\end{table}

\paragraph{Hardware \& Runtime.} We run all experiments on a NVIDIA Quadro RTX 6000 GPU (24 GB of memory). The single image fitting and regularization experiments require approximately 1 hour to run.
