# Supplementary material for: Implicit Neural Representations with Periodic Activation Functions
Source: arXiv:2006.09661 source file (2020-06-17)
Supplement: Supplementary file 3 [file supplement_audio.tex]

Various methods exist for audio signal representation. Early work consists of representing audio signals using various spectral features~\cite{NIPS2009_3674, bertrand2008specfeat, kong2018audio}. Spectrograms, representations of the spectrum of frequencies of a signal as it varies with time, have been used in machine learning applications due to the ease of applying widely successful image processing CNN architectures to them~\cite{hershey2017audio, donahue2019wavegan, shen2018spectrogram}. More recently, neural network architectures have been developed which can operate on raw audio waveforms~\cite{oord2016wavenet, donahue2019wavegan, mehri2016samplernn}. 

To demonstrate the versatility of \sinet{}s as implicit neural representations, we show that they can efficiently model audio signals. Due to the highly periodic nature of audio signals with structure at various time scales, we expect that \sinet{}s could accurately represent such signals efficiently and provide an alternative representation for audio signals.
We evaluate \sinet{} performance on raw audio waveforms of varying length clips of music and speech. While other neural network architectures fail to accurately model waveforms, \sinet{}s are able to quickly converge to a representation which can be replayed with minimal distortion. We fit a \sinet{} to a sampled waveform $a$ using a loss of the form:
\begin{equation}
	\mathcal{L} = \int_\Omega \| \Sha_a (\implicit(\mathbf{x})) - a(\mathbf{x}) \|^2\, d\mathbf{x}.
\end{equation}
where $\Sha_a$ samples the \sinet{} at the waveform measurement locations. 

\begin{figure}[t!]
	\includegraphics[width=\textwidth]{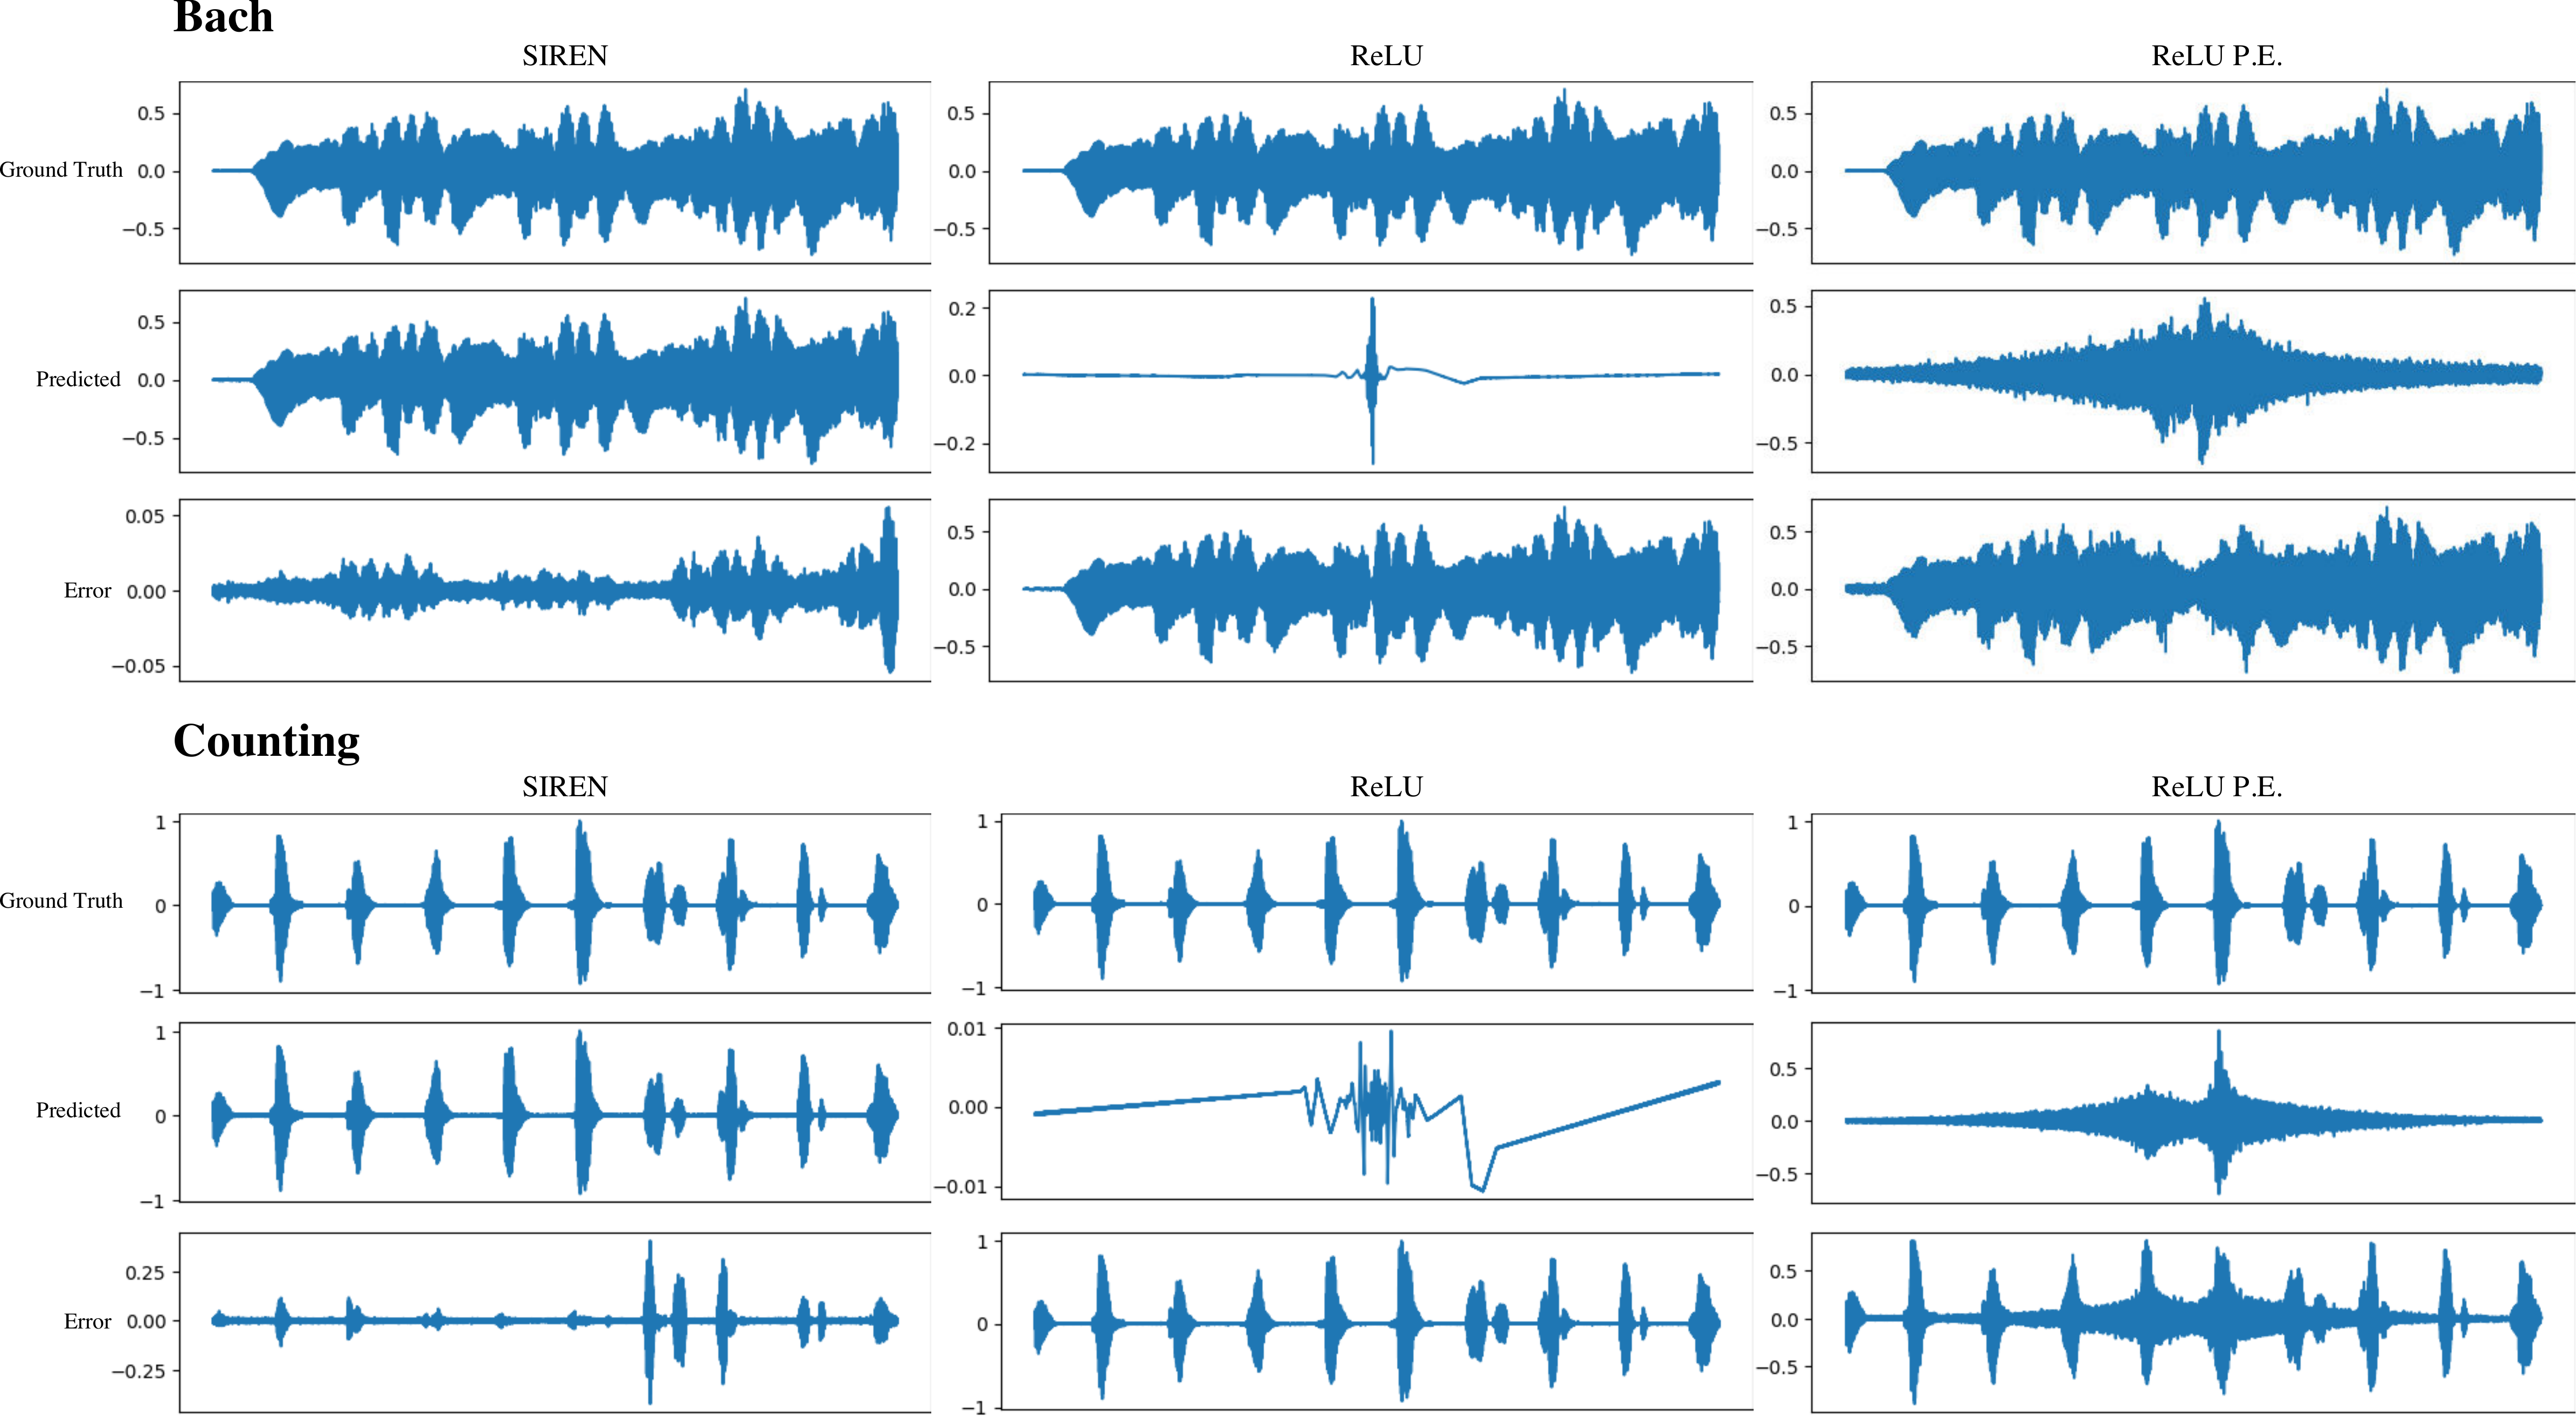}
	\caption{Fitted waveforms and error for various implicit neural representation architectures. We fit the network to the first 7 seconds of Bach's Cello Suite No. 1: Prelude (Bach) and to a 12 second clip of a male actor counting 0-9 (Counting). Only \sinet{} representations capture the waveform structure.}
	\label{fig:audio}
\end{figure}

Fig.~\ref{fig:audio} displays the fit waveform to music and speech data respectively. We see that other neural network architectures are not able to represent raw audio waveforms at all, while \sinet{}s produce an accurate waveform. Additionally, we note that the number of parameters in out \sinet{} is far less than the number of samples in the ground truth waveform. This ability to compress signals supports our claim that periodic \sinet{} representations are well suited to representing audio signals, and perhaps lossy compression algorithms for audio could be designed using \sinet{}s. Our supplemental video contains audio from the \sinet{}, which is accurate and recognizable.
Tab.~\ref{tab:audio_MSE} shows the converged \sinet{} mean-squared error on the original audio signal and statistics on these metrics (these were feasible to evaluate due to the relatively short training time of \sinet{}s on audio signals). This shows \sinet{}s are highly stable in convergence.

\begin{table}
	\vspace{-.3cm}
	\caption{Mean squared error of representing the raw audio waveform scaled in the range $[-1,1]$ with a \sinet{}. The mean and variance of the reconstruction MSE are evaluated over $10$ independent runs of fitting. Each architecture is fitted for $5000$ iterations.}
	\label{tab:audio_MSE}
	\centering
	\begin{tabular}{lcccc}
		\toprule
		& Bach & Bach & Counting & Counting \\
		Architecture & MSE Mean & MSE Standard Dev. & MSE Mean & MSE Standard Dev. \\
		\midrule
		ReLU & $2.504\times10^{-2}$ & $1.706\times10^{-3}$ & $7.466\times10^{-3}$ & $8.217\times10^{-5}$ \\ 
		ReLU P.E. & $2.380\times10^{-2}$ & $3.946\times10^{-4}$ & $9.078\times10^{-3}$ & $9.627\times10^{-4}$ \\ 
		\sinet{} & $1.101\times10^{-5}$ & $2.539\times10^{-6}$ & $3.816\times10^{-4}$ & $1.632\times10^{-5}$ \\ 
		\bottomrule
	\end{tabular}
\end{table}

\subsection{Reproducibility \& Implementation Details}
\paragraph{Data.} For music data, we use the first 7 seconds from Bach's Cello Suite No. 1: Prelude available at \url{https://www.yourclassical.org/story/2017/04/04/daily-download-js-bach--cello-suite-no-1-prelude} and for the speech we use stock audio of a male actor counting from 0 to 9 available at \url{http://soundbible.com/2008-0-9-Male-Vocalized.html}. These waveforms are have a sampling rate of 44100 samples per second. As pre-processing, they are normalized to be in the range of $[-1,1]$. We use the entire set of samples to fit our \sinet{} in each batch.

\paragraph{Architecture.} We use the same 5-layer MLP with sine nonlinearities as for all other \sinet{} applications. 

\paragraph{Frequency Scaling.}
To account for the high sampling rate of audio signals, we scale the domain $\mathbf{x}\in [-100, 100]$ instead of $[-1,1]$. This is equivalent to adding a constant multiplication term to the weights of the input layer of the \sinet{}.

\paragraph{Hyperparameters.} We use the Adam optimizer with a learning rate of $5\times10^{-5}$ to generate the results. We evaluated both learning rates of $5\times10^{-5}$ and $1\times10^{-4}$, finding that $5\times10^{-5}$ worked slightly better. We train for 9,000 iterations for the figures generated, and 5,000 iterations for the quantitative results listen in the table (the model is largely converged after only 2,000 iterations).

\paragraph{Hardware \& Runtime.} The experiments are conducted on a NVIDIA Quadro RTX 6000 GPU (24 GB of memory), where training for $9000$ iterations takes roughly 20 minutes for the Bach signal and 30 minutes for the counting signal.
