# Supplementary material for: Implicit Neural Representations with Periodic Activation Functions
Source: arXiv:2006.09661 source file (2020-06-17)
Supplement: Supplementary file 4 [file supplement_derivative.tex]

\newcommand{\weights}[1]{\mathbf{W}_{#1}}
\newcommand{\tweights}[1]{\hat{\mathbf{W}}_{#1}}

\newcommand{\tcoords}{\hat{\coords}}

\newcommand{\bias}[1]{\mathbf{b}_{#1}}
\newcommand{\sinel}[1]{\phi_{#1}}

\newcommand{\linear}[1]{\mathbf{T}_{#1}}

\newcommand{\tweightst}[1]{\hat{\mathbf{W}}_{#1}^T}

\newcommand{\cweights}[1]{\check{\mathbf{W}}_{#1}}

\newcommand{\acts}[1]{\mathbf{y}_{#1}}
\newcommand{\cacts}[1]{\check{\mathbf{y}}_{#1}}

\newcommand{\deriv}[2]{\frac{\partial{#1}}{\partial{#2}}}

We can write a loss $L$ between a $\mathrm{target}$ and a \sinet{} output as:
\begin{equation}
    L\big(\mathrm{target},(\weights{n}\circ\sinel{n-1}\circ\sinel{n-2}\ldots\sinel{0})(\coords)+\bias{n}\big).
\end{equation}
A sine layer is defined as:
\begin{equation}
    \sinel{i}(\coords) = (\sin\circ\linear{i})(\coords),\quad 
    \text{with } \linear{i}: \coords\mapsto \weights{i}\coords + \bias{i} = \tweights{i}\tcoords,
\end{equation}
defining $\tweights{}=[\weights{},\bias{}]$ and $\tcoords=[\coords,1]$ for convenience.

The gradient of the loss with respect to the input can be calculated using the chain rule:
\begin{align}
    \nabla_\coords L 
    &= \Big(   \deriv{L}{\acts{n}}\cdot\deriv{\acts{n}}{\acts{n-1}}\cdot
        \ldots\deriv{\acts{1}}{\acts{0}}\cdot\deriv{\acts{0}}{\coords}  \Big)^T \nonumber \\
    &= (\tweightst{0}\cdot \sin'(\acts{0}))\cdot\ldots\cdot(\tweightst{n-1}\cdot\sin'(\acts{n-1}))\cdot\tweightst{n}\cdot L'(\acts{n})
    \label{eq:chain_rule_sinenet}
\end{align}

where $\acts{l}(\tcoords)$ is defined as the network evaluated on input $\tcoords$ stopping before the non-linearity of layer $l$, ($\tcoords$ is implicit in Equation~\eqref{eq:chain_rule_sinenet} for the sake of readability):
\begin{align}
    \acts{0}(\tcoords) 
    &= \tweights{0}\tcoords \nonumber \\
    \acts{l}(\tcoords) 
    &=  (\tweights{l}\circ\sin) (\acts{l-1})
    = (\tweights{l}\circ\sin\circ\ldots \tweights{0})(\tcoords)
\end{align}
Remarking that the derivative $\sin'(\acts{l})=\cos(\acts{l})=\sin(\acts{l}+\frac{\pi}{2})$, and that we can absorb the $\frac{\pi}{2}$ phase offset in the bias by defining the new weight matrix $\cweights{} = [\weights{},\bias{}+\frac{\pi}{2}]$. The gradient can be rewritten:
\begin{align}
\nabla_\coords L =
(\tweightst{0}\cdot \sin(\cacts{0}))\cdot\ldots\cdot(\tweightst{n-1}\cdot\sin(\cacts{n-1}))\cdot\tweightst{n}\cdot L'(\acts{n})
\label{eq:grad_sinet}
\end{align}
with $\cacts{l}$ the activations using the weights $\cweights{l}$
\begin{align}
    \cacts{0}(\tcoords) 
    &= \cweights{0}\tcoords \nonumber \\
    \cacts{l}(\tcoords) 
    &=  (\cweights{l}\circ\sin) (\acts{l-1})
    = (\cweights{l}\circ\sin\circ\ldots \cweights{0})(\tcoords)
\end{align}
which is a forward pass evaluating a slightly different \sinet{} in which all the biases have been shifted by $\frac{\pi}{2}$.

Furthermore, in Equation~\eqref{eq:grad_sinet} since every term of the form $\sin(\acts{l})$ is a \sinet{}, and those terms are multiplied by weight matrices between them, this shows that the gradient of a \sinet{} can be evaluated by yet another \sinet{}. It also shows that a \sinet{} of L layers, requires the evaluation of a \sinet{} of $\frac{L\cdot(L+1)}{2}$ layers.
