# Supplementary material for: Implicit Neural Representations with Periodic Activation Functions
Source: arXiv:2006.09661 source file (2020-06-17)
Supplement: Supplementary file 5 [file supplement_generalization.tex]

A strong prior over the space of \sinet{} functions enables applications such as reconstruction from noisy or few observations. We demonstrate that this can be done over the function space of \sinet{}s representing faces in the CelebA dataset~\cite{liu2015faceattributes}. We use the learned prior to perform image inpainting of missing pixels.

\subsection{Reproducibility \& Implementation Details}

\paragraph{Data.} Partial observations (referred to as context) of the input image consist of coordinates and pixel values $\context=\{(x_i,c_i)\}_{i=0}^N$ sampled from an image $\lowresimg\in\mathbb{R}^{H\times W\times 3}$. Like in ~\cite{garnelo2018conditional}, $\lowresimg\in\mathbb{R}^{32\times 32\times 3}$ is center-cropped and downsampled from the images in the CelebA training dataset, containing 162,770 images. We evaluate our test performance on a similarly center-cropped and downsampled version of the CelebA test dataset, containing 19,962 images.

\paragraph{Context Encoder.} The results presented in the main paper use a convolutional neural network encoder which operates on sparse images. More specifically, the partial observations are combined into sparse images $\context\in\mathbb{R}^{32\times 32\times 3}$, where observed pixel locations are either their value $c_i$ and masked pixel locations are given a value of $0$.
The encoder $\encoder$ operates on these sparse images, and is parameterized as a standard convolutional neural network (CNN) with an input convolutional layer followed by four residual blocks with ReLU nonlinearities. Each intermediate feature map has $256$ channels. 
This outputs per-pixel embeddings in $\mathbb{R}^{256}$, which are aggregated together into a single context embedding using a fully connected layer. 

We also describe the use of a set encoder as in ~\cite{garnelo2018conditional} for encoding the partial observations. In this case, partial observations consist of a list of coordinates and pixel values $\context=\{(x_i, c_i)\}_{i=0}^N, (x_i, c_i)\in\mathbb{R}^5$.
The encoder $\encoder$ is an MLP which operates on each of these observations independently. The MLP consists of two hidden layers with sine nonlinearities, and outputs an embedding per pixel in $\mathbb{R}^{256}$.
The embeddings are aggregated together using a mean operation. Since each embedding depends only on the context pixel, and the mean operation is symmetric, this set encoder is permutation invariant.  

We consider one final encoder $\encoder$ based on partial convolutions~\cite{Liu2018ECCV}. Partial convolutions are designed to operate on sparse images, conditioning outputs of each layer only on valid input pixels. In this case, the partial observations are combined into a sparse image and mask, much like in the CNN encoder case.
However, the encoder is implemented using an input partial convolution followed by four partial convolution residual layers with ReLU nonlinearities. Each intermediate map also has $256$ channels. The output per-pixel embeddings are similarly aggregated togheter into a single context embedding using a fully connected layer.

\paragraph{Hypernetwork.} We use a hypernetwork as our decoder, which maps the latent code to the weights of a 5-layer \sinet{} with hidden features of size $256$ (as in all other experiments). This hypernetwork is a ReLU MLP with one hidden layer with $256$ hidden features.

\paragraph{Loss Function.} We train the encoder $\encoder$ and hypernetwork $\hypernet$ operating on context $\context$  by minimizing the loss function:
\begin{align}
	\loss = \underbrace{\frac{1}{HW}\lVert\implicit(\mathbf{x}) - \lowresimg\rVert_2^2}_{\loss_{\text{img}}} + \lambda_1\underbrace{\frac{1}{k}\lVert \latentcode \rVert^2_2}_{\loss_{\text{latent}}} + \lambda_2\underbrace{\frac{1}{l}\lVert \implicitparams \rVert_2^2}_{\loss_{\text{weights}}}
\end{align}
where $(H,W)$ are the spatial dimensions of the images in the dataset, $\implicit=(\hypernet\circ\encoder)(\context)$ is the predicted \sinet{} representation from the hypernetwork, $\lowresimg$ is the ground truth image, $k$ is the dimensionality of the embedding $\latentcode$, and $l$ is the amount of weights $\implicit$ in the \sinet{} $\implicit$.

$\loss_{\text{img}}$ enforces the closeness of image represented by the \sinet{} to ground-truth, $\loss_{\text{latent}}$ enforces a Gaussian prior on latent code $\latentcode$, and $\loss_{\text{weights}}$ is a regularization term on the weights of $\implicit$ which can be interpreted as encouraging a lower frequency representation of the image. The regularization terms are necessary since there are many possible \sinet{} representations for an image, so we need to encourage unique solutions (lowest possible frequency) which lie in a more compact latent space (Gaussian).
For all of our results, we use regularization weighting parameters of $\lambda_1=1\times 10^{-1}$ and $\lambda_2=1\times 10^{2}$. 

\paragraph{Hypernetwork Initialization.} In order to improve performance, we devise a heuristic initialization scheme for the hypernetwork which deviates from the default Kaiming initialization for ReLU MLP networks~\cite{he2015delving}. Although a formal theoretical analysis of this initialization has not been well studied, we found that the initialization led to convergence of our encoder and hypernetwork models. 
We only modify the default ReLU MLP initialization in the final layer of the hypernetwork by scaling the Kaiming initialized weights by $1\times10^{-2}$, and initializing the biases uniformly in the range of $[-1/n, 1/n]$ where $n$ is the number of inputs to the layer of the \sinet{} being predicted. 

The motivation for this scheme is that the initialization of the biases of the hypernetwork is a heuristic initialization of \sinet{}s which leads to high quality convergence results. Thus, initializing the weights of the hypernetwork with a small magnitude ensures that the \sinet{} weights outputted at initialization of the hypernetwork are close to a initialization of a single \sinet{}, regardless of input to the hypernetwork.

\paragraph{Training Procedure.} In order to encourage invariance to the number of partial observations, we randomly sample from $10$ to $1000$ context pixels to input into the convolutional or partial convolutional encoder. In the case of the set encoder which is permutation invariant, we mimic the training procedure of ~\cite{garnelo2018conditional} by varying from $10$ to $200$ sampled context pixels.

\paragraph{Hyperparameters.} As mentioned, we use loss parameters $\lambda_1=1\times 10^{-1}$ and $\lambda_2=1\times 10^{2}$. For all experiments, we use the Adam optimizer with a learning rate of $5\times 10^{-5}$, a batch size of 200 images, and train for 175 epochs on the training dataset. We found these hyperparameters by trial and error, having tested values of $\lambda_1\in[10^{-3}, 10^{-1}]$, $\lambda_2\in[10^{1}, 10^{4}]$, learning rates of $5\times 10^{-5}, 1\times 10^{-4}$, and a batch size of 200 and 1000. 

\paragraph{Runtime.} We train the videos for 175 epochs on the downsampled CelebA training set, requiring approximately 24 hours.

\paragraph{Hardware.} The networks are trained using NVIDIA Quadro RTX 6000 GPUs with 24 GB of memory.

\subsection{Additional Results}
We show additional results from the convolutional encoder in Fig.~\ref{fig:generalization_conv_additional}

\begin{figure}
	\centering
	\includegraphics[width=.85\textwidth]{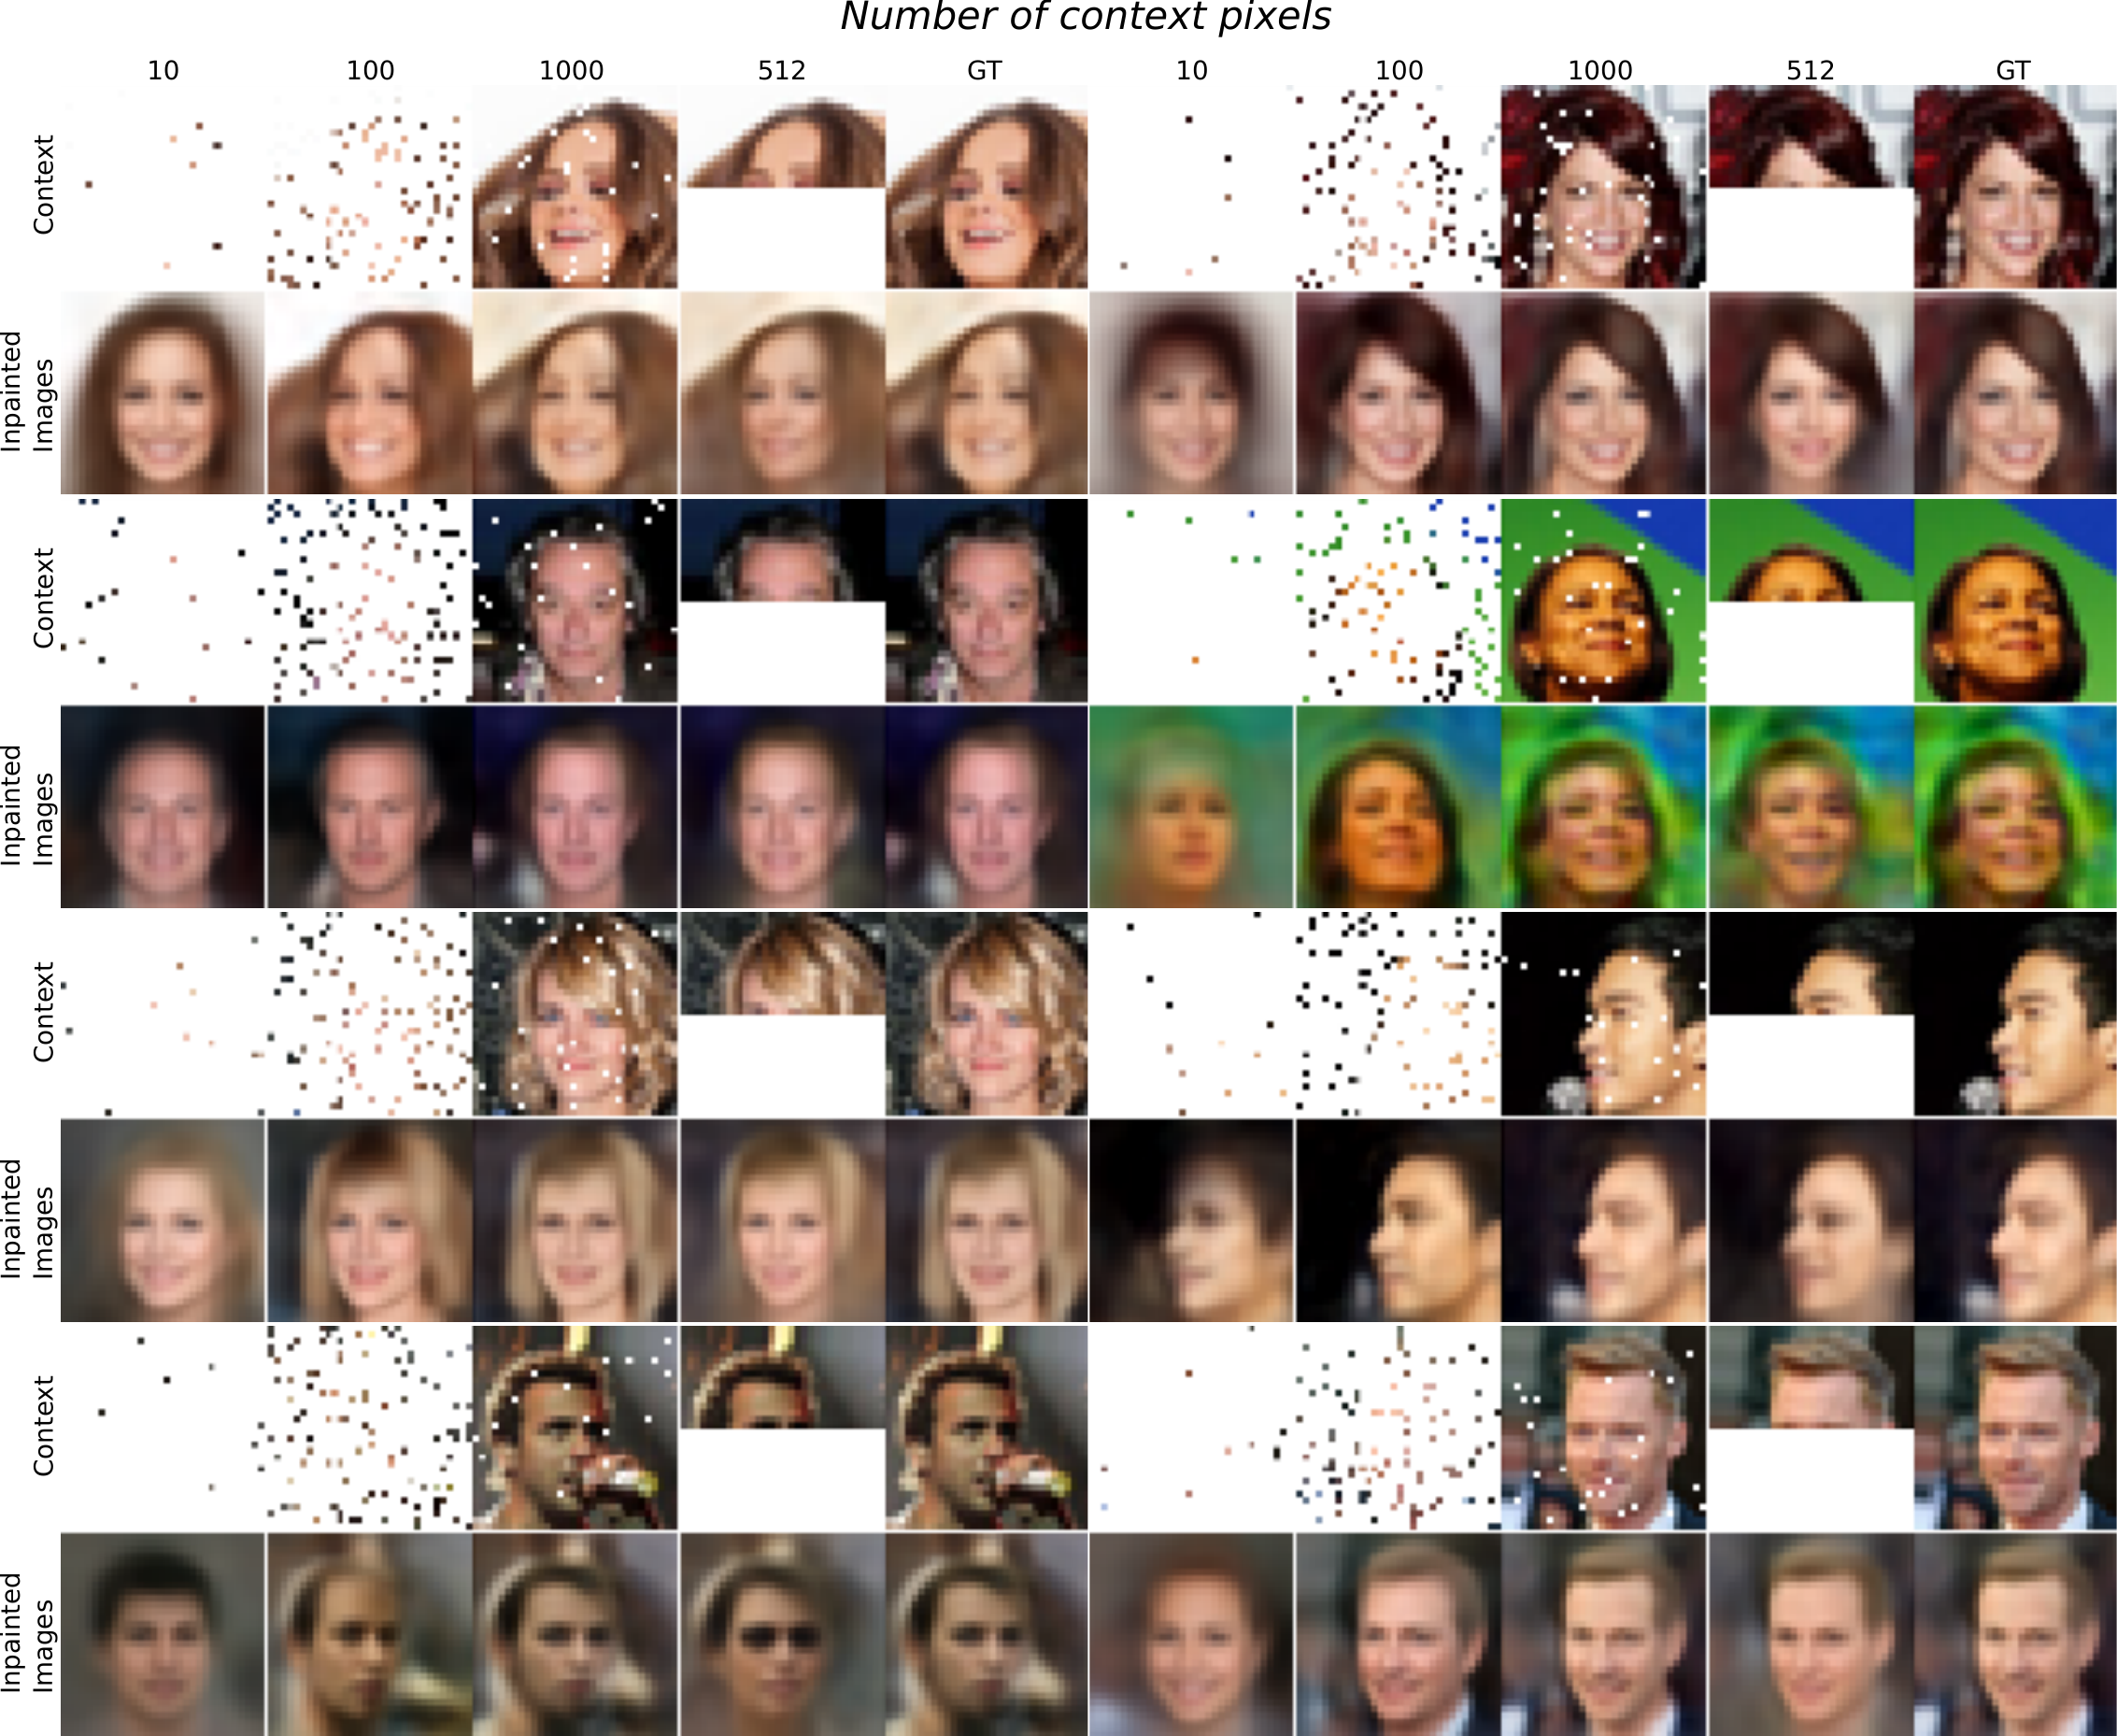} 
	\caption{Additional results using the CNN encoder with hypernetwork decoder.}
	\label{fig:generalization_conv_additional}
\end{figure}

We also show results from the set encoder with sine nonlinearities in Fig.~\ref{fig:generalization_cnp}, set encoder with ReLU nonlinearities (as in the original CNP architecture) in Fig.~\ref{fig:generalization_cnp_relu}, and convolutional encoder based on partial convolutions in Fig.~\ref{fig:generalization_partial_conv}. All of these implementations use the same hypernetwork architecture as a decoder from latent codes to \sinet{} weights. Tab.~\ref{tab:generalization_additional} shows comparisons between architectures for the encoder.

Interestingly, the partial convolutional encoder performs worse than both the set encoders and convolutional encoder. We suspect that the convolutional encoder has an easier time capturing complex spatial relationships between the context pixels and using information from the masked pixels instead of only conditioning on valid pixels. Regardless of encoder architecture, some prior over the space of \sinet{}s has been learned which can be used to perform inpainting comparably to methods such as CNP~\cite{garnelo2018conditional} operating on images directly.

\begin{figure}
	\centering
	\includegraphics[width=.85\textwidth]{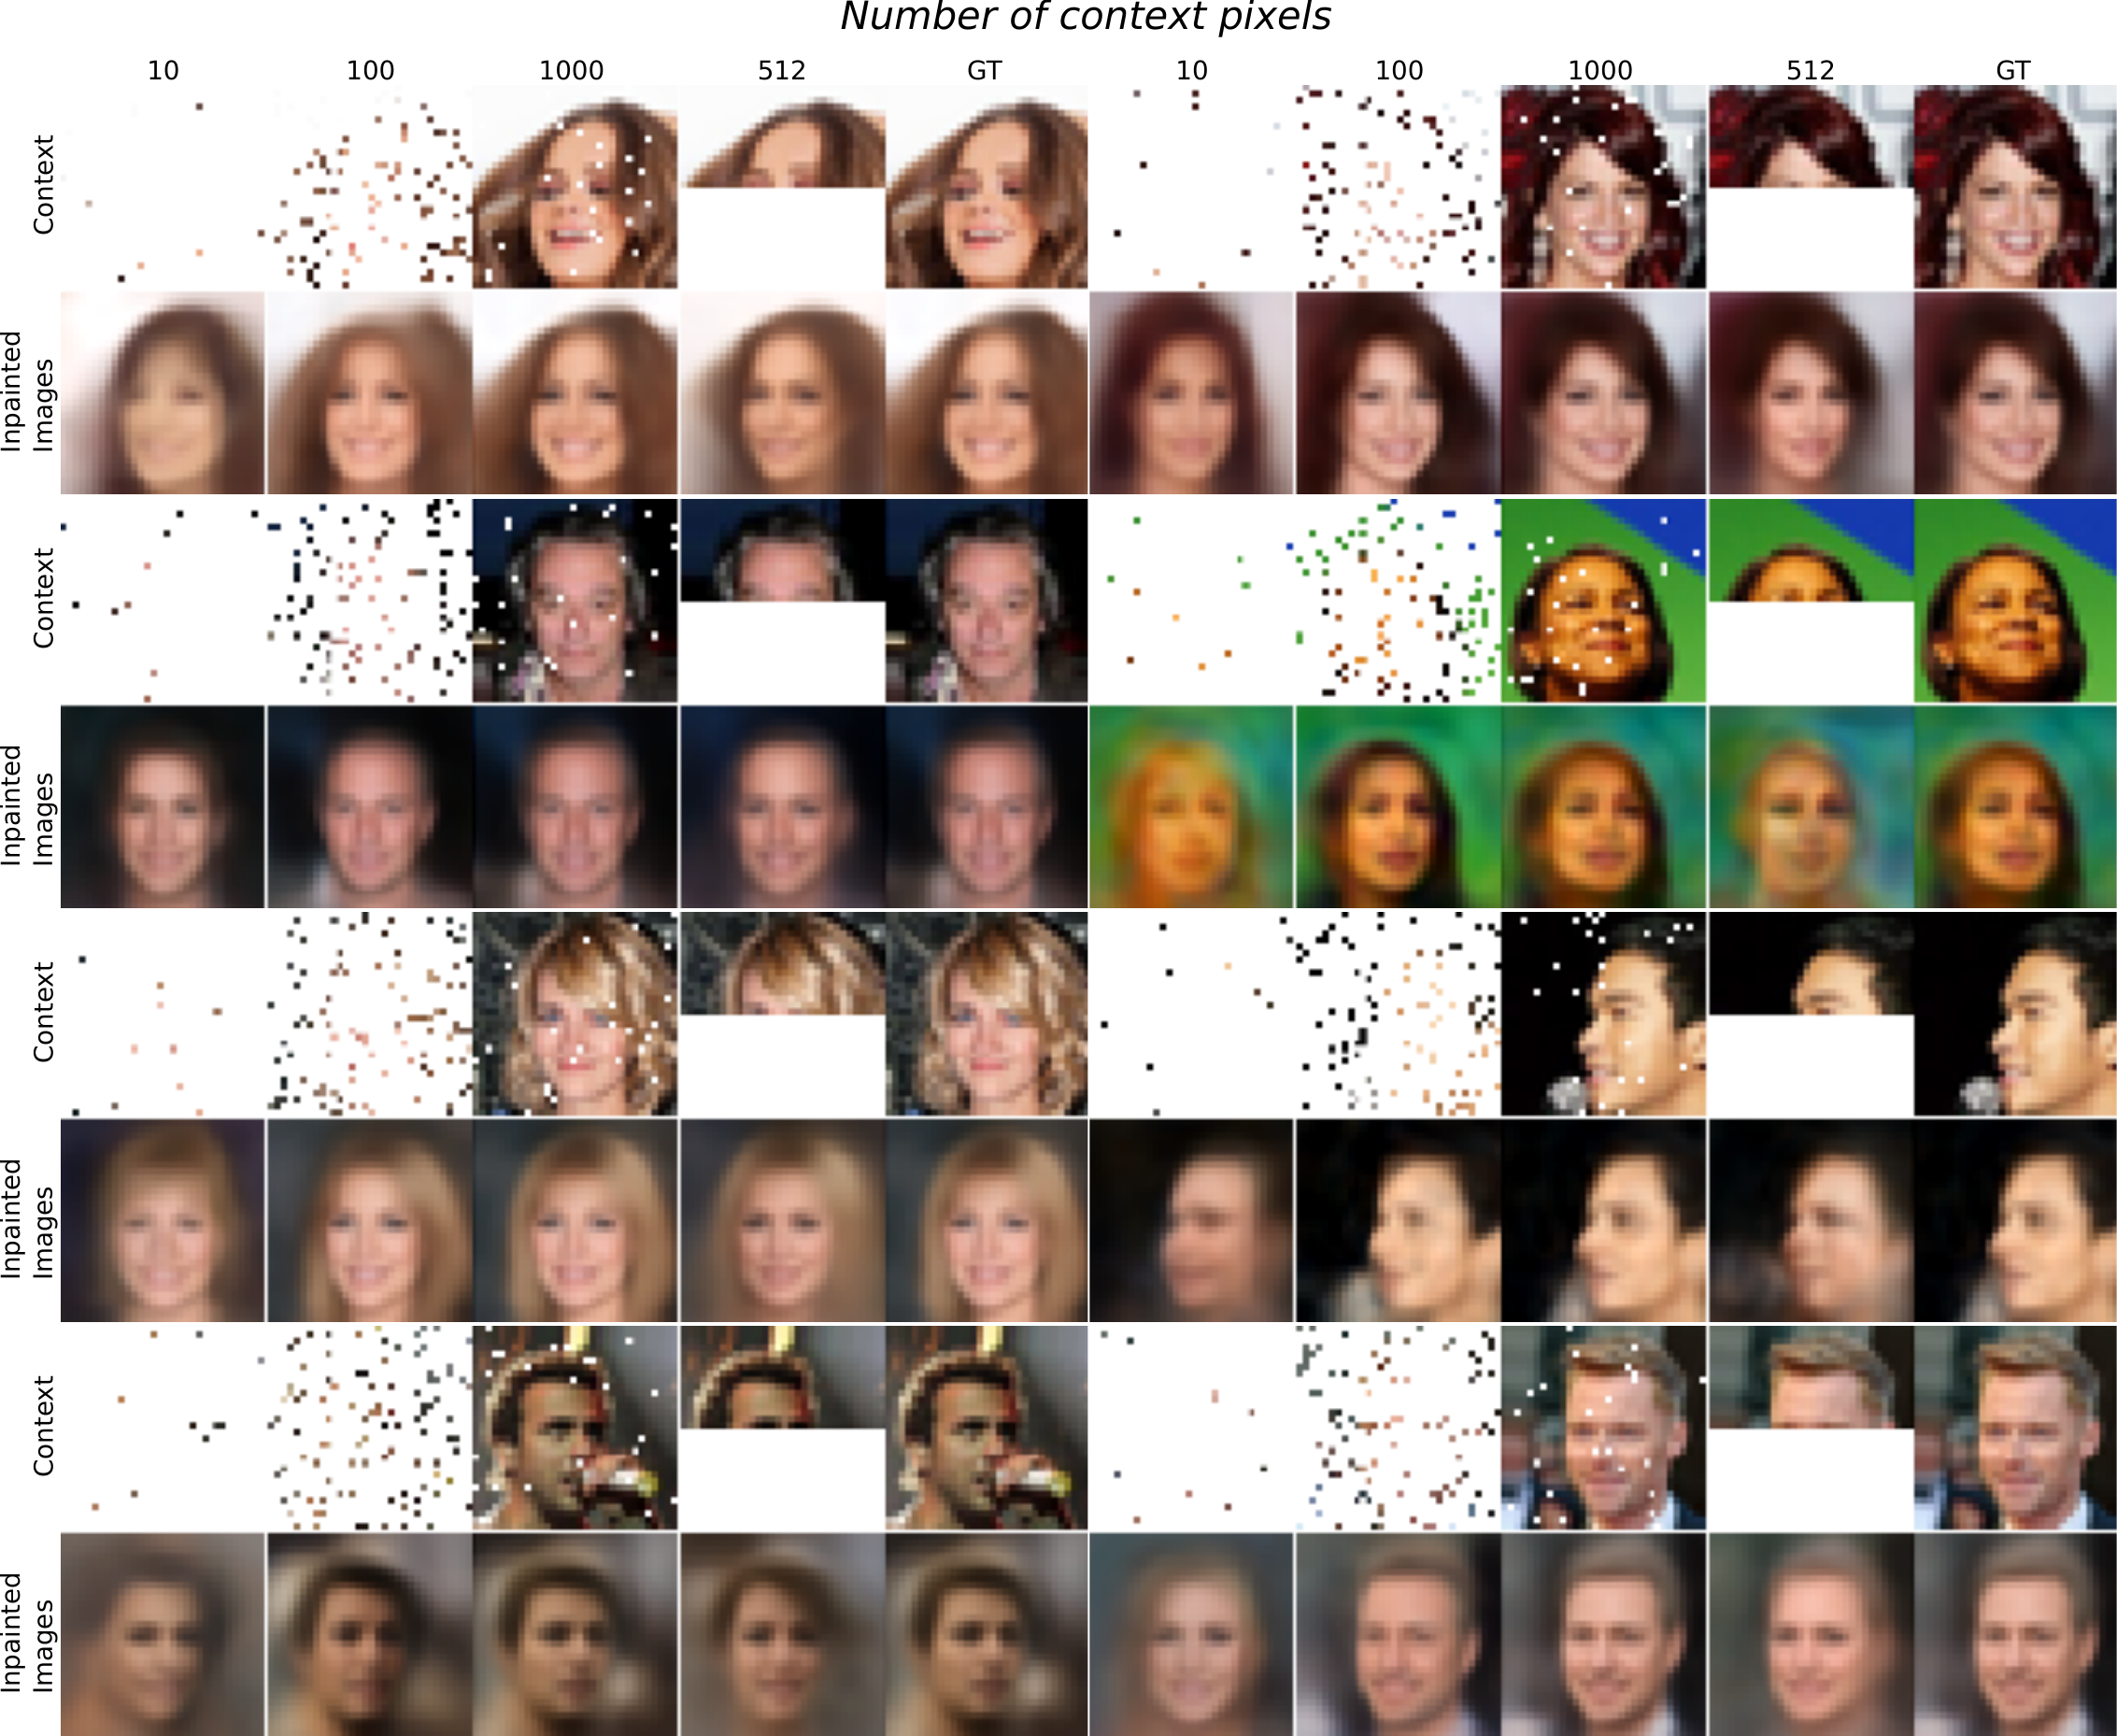}
	\caption{Additional results using the set encoder with sine nonlinearities with a hypernetwork decoder.}
	\label{fig:generalization_cnp}
\end{figure}

\begin{figure}
	\centering
	\includegraphics[width=.85\textwidth]{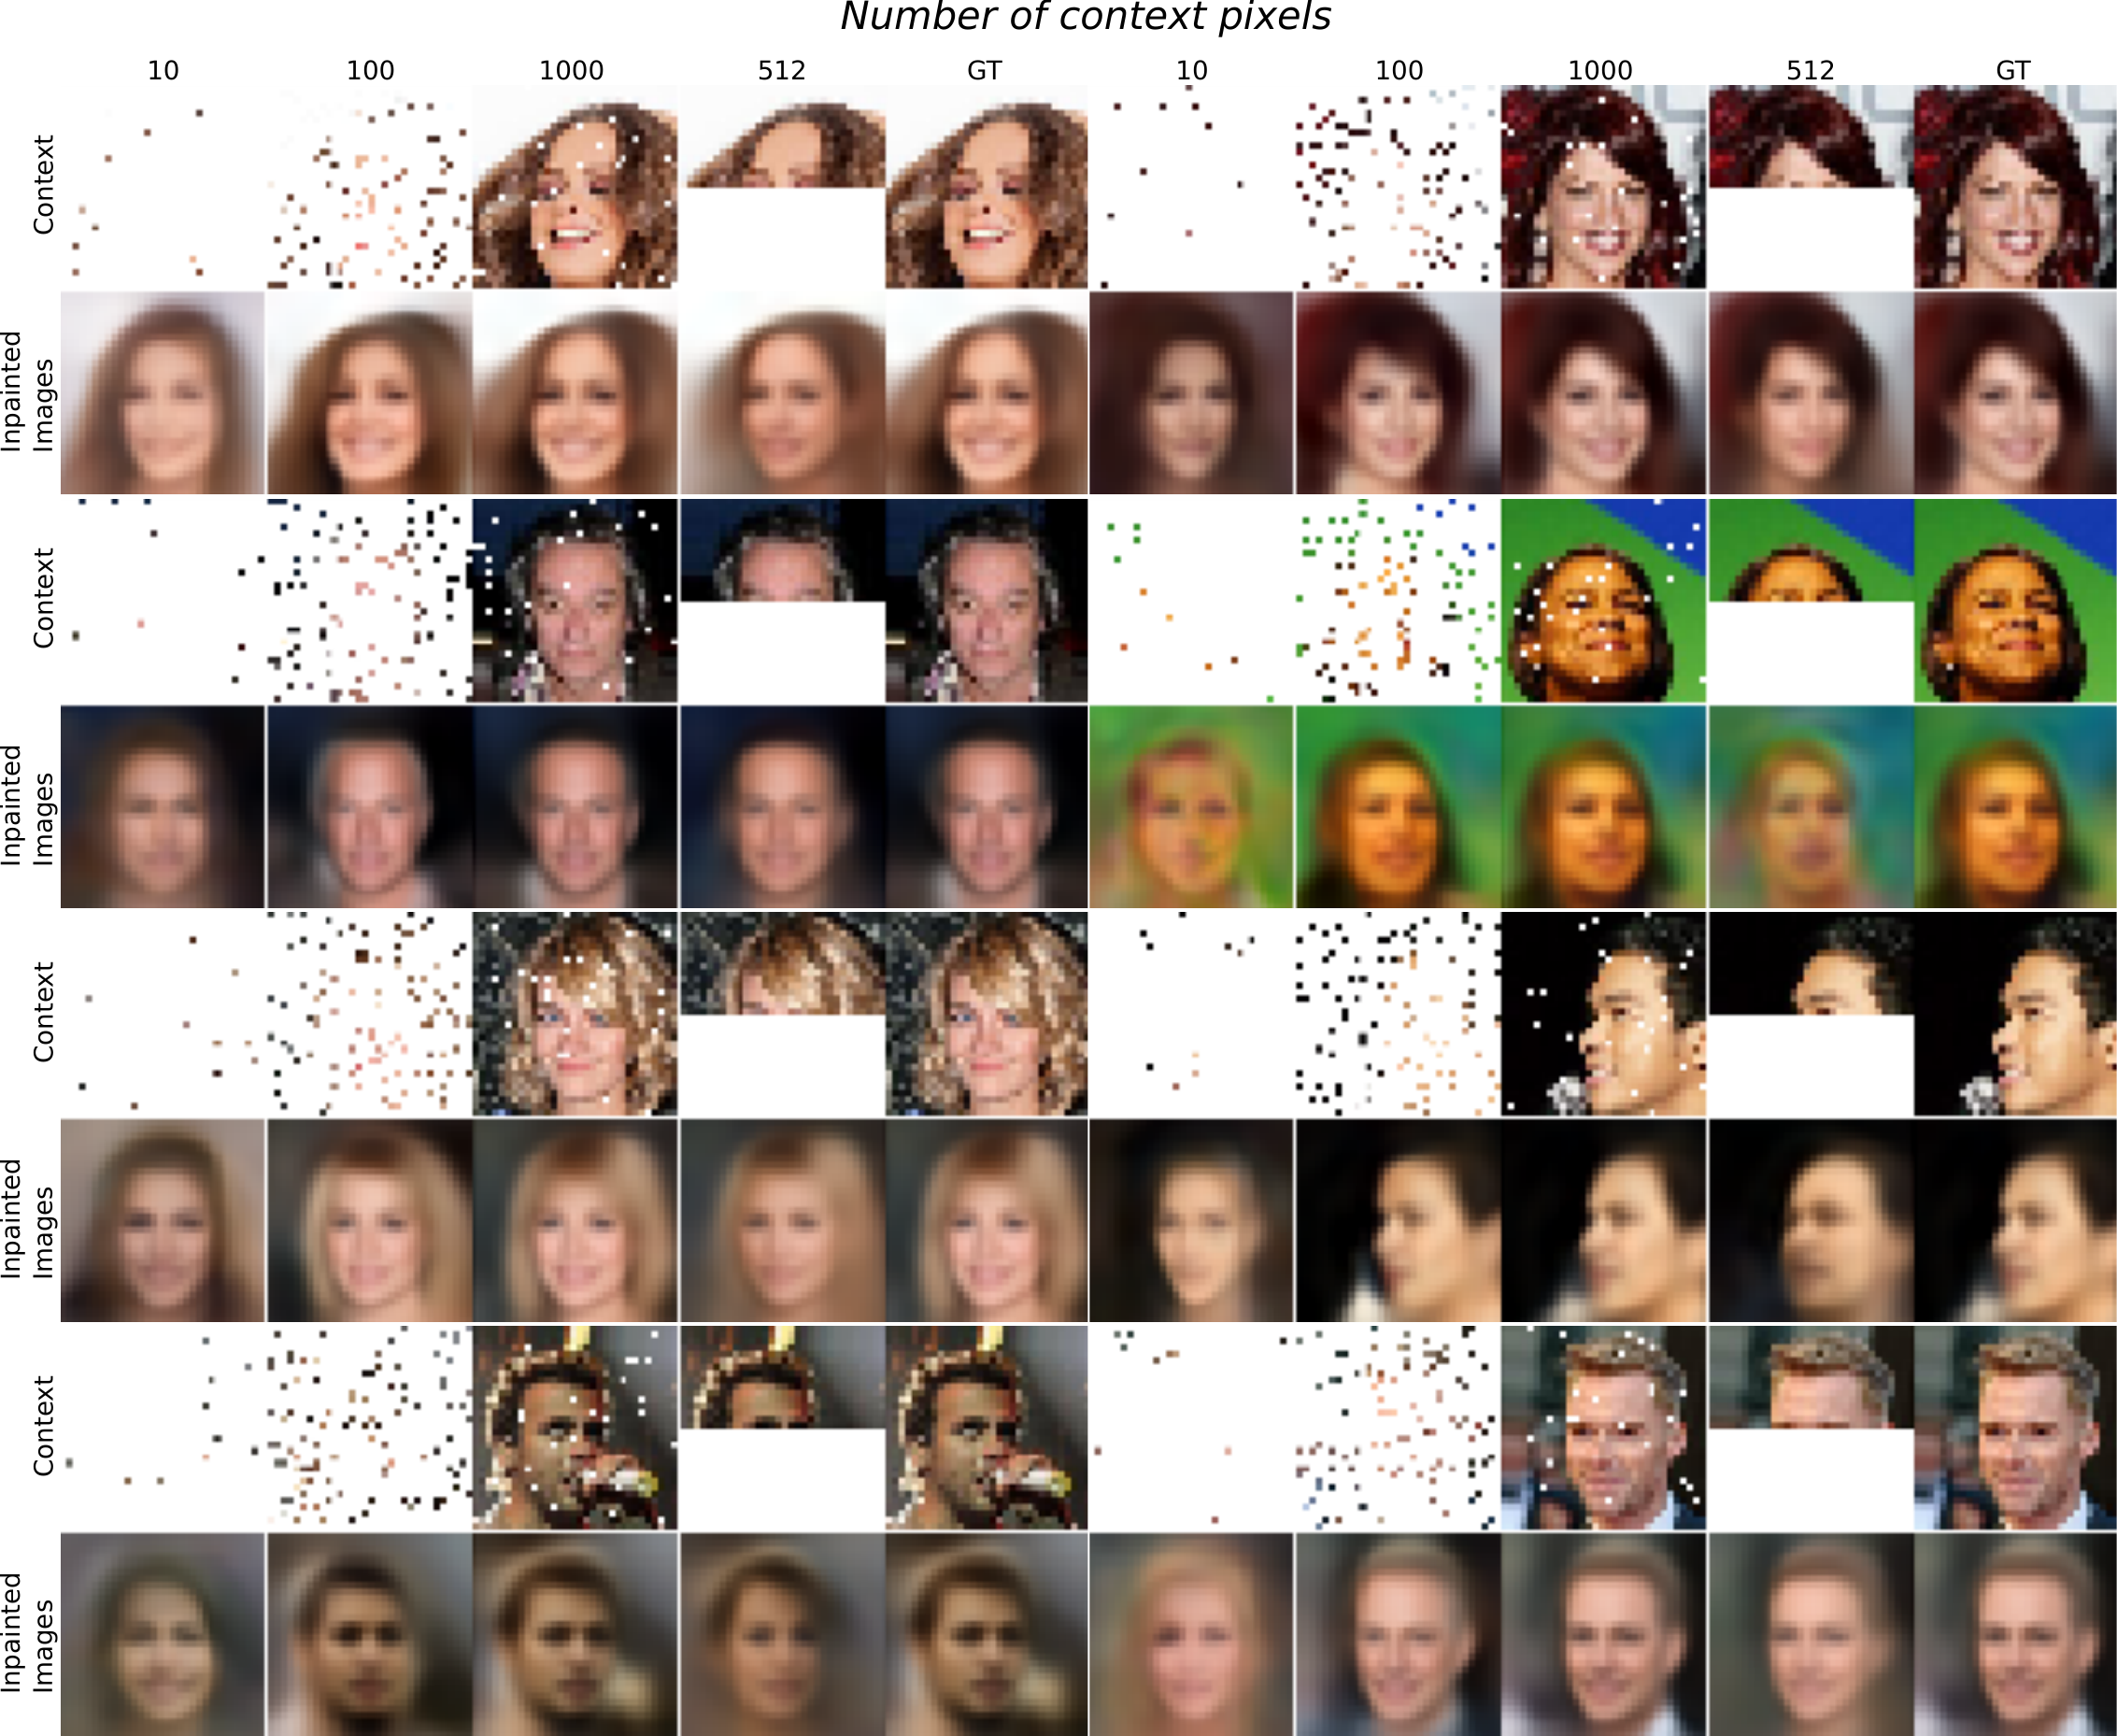}
	\caption{Additional results using the set encoder with ReLU nonlinearities with a hypernetwork decoder.}
	\label{fig:generalization_cnp_relu}
\end{figure}

\begin{figure}
	\centering
	\includegraphics[width=.85\textwidth]{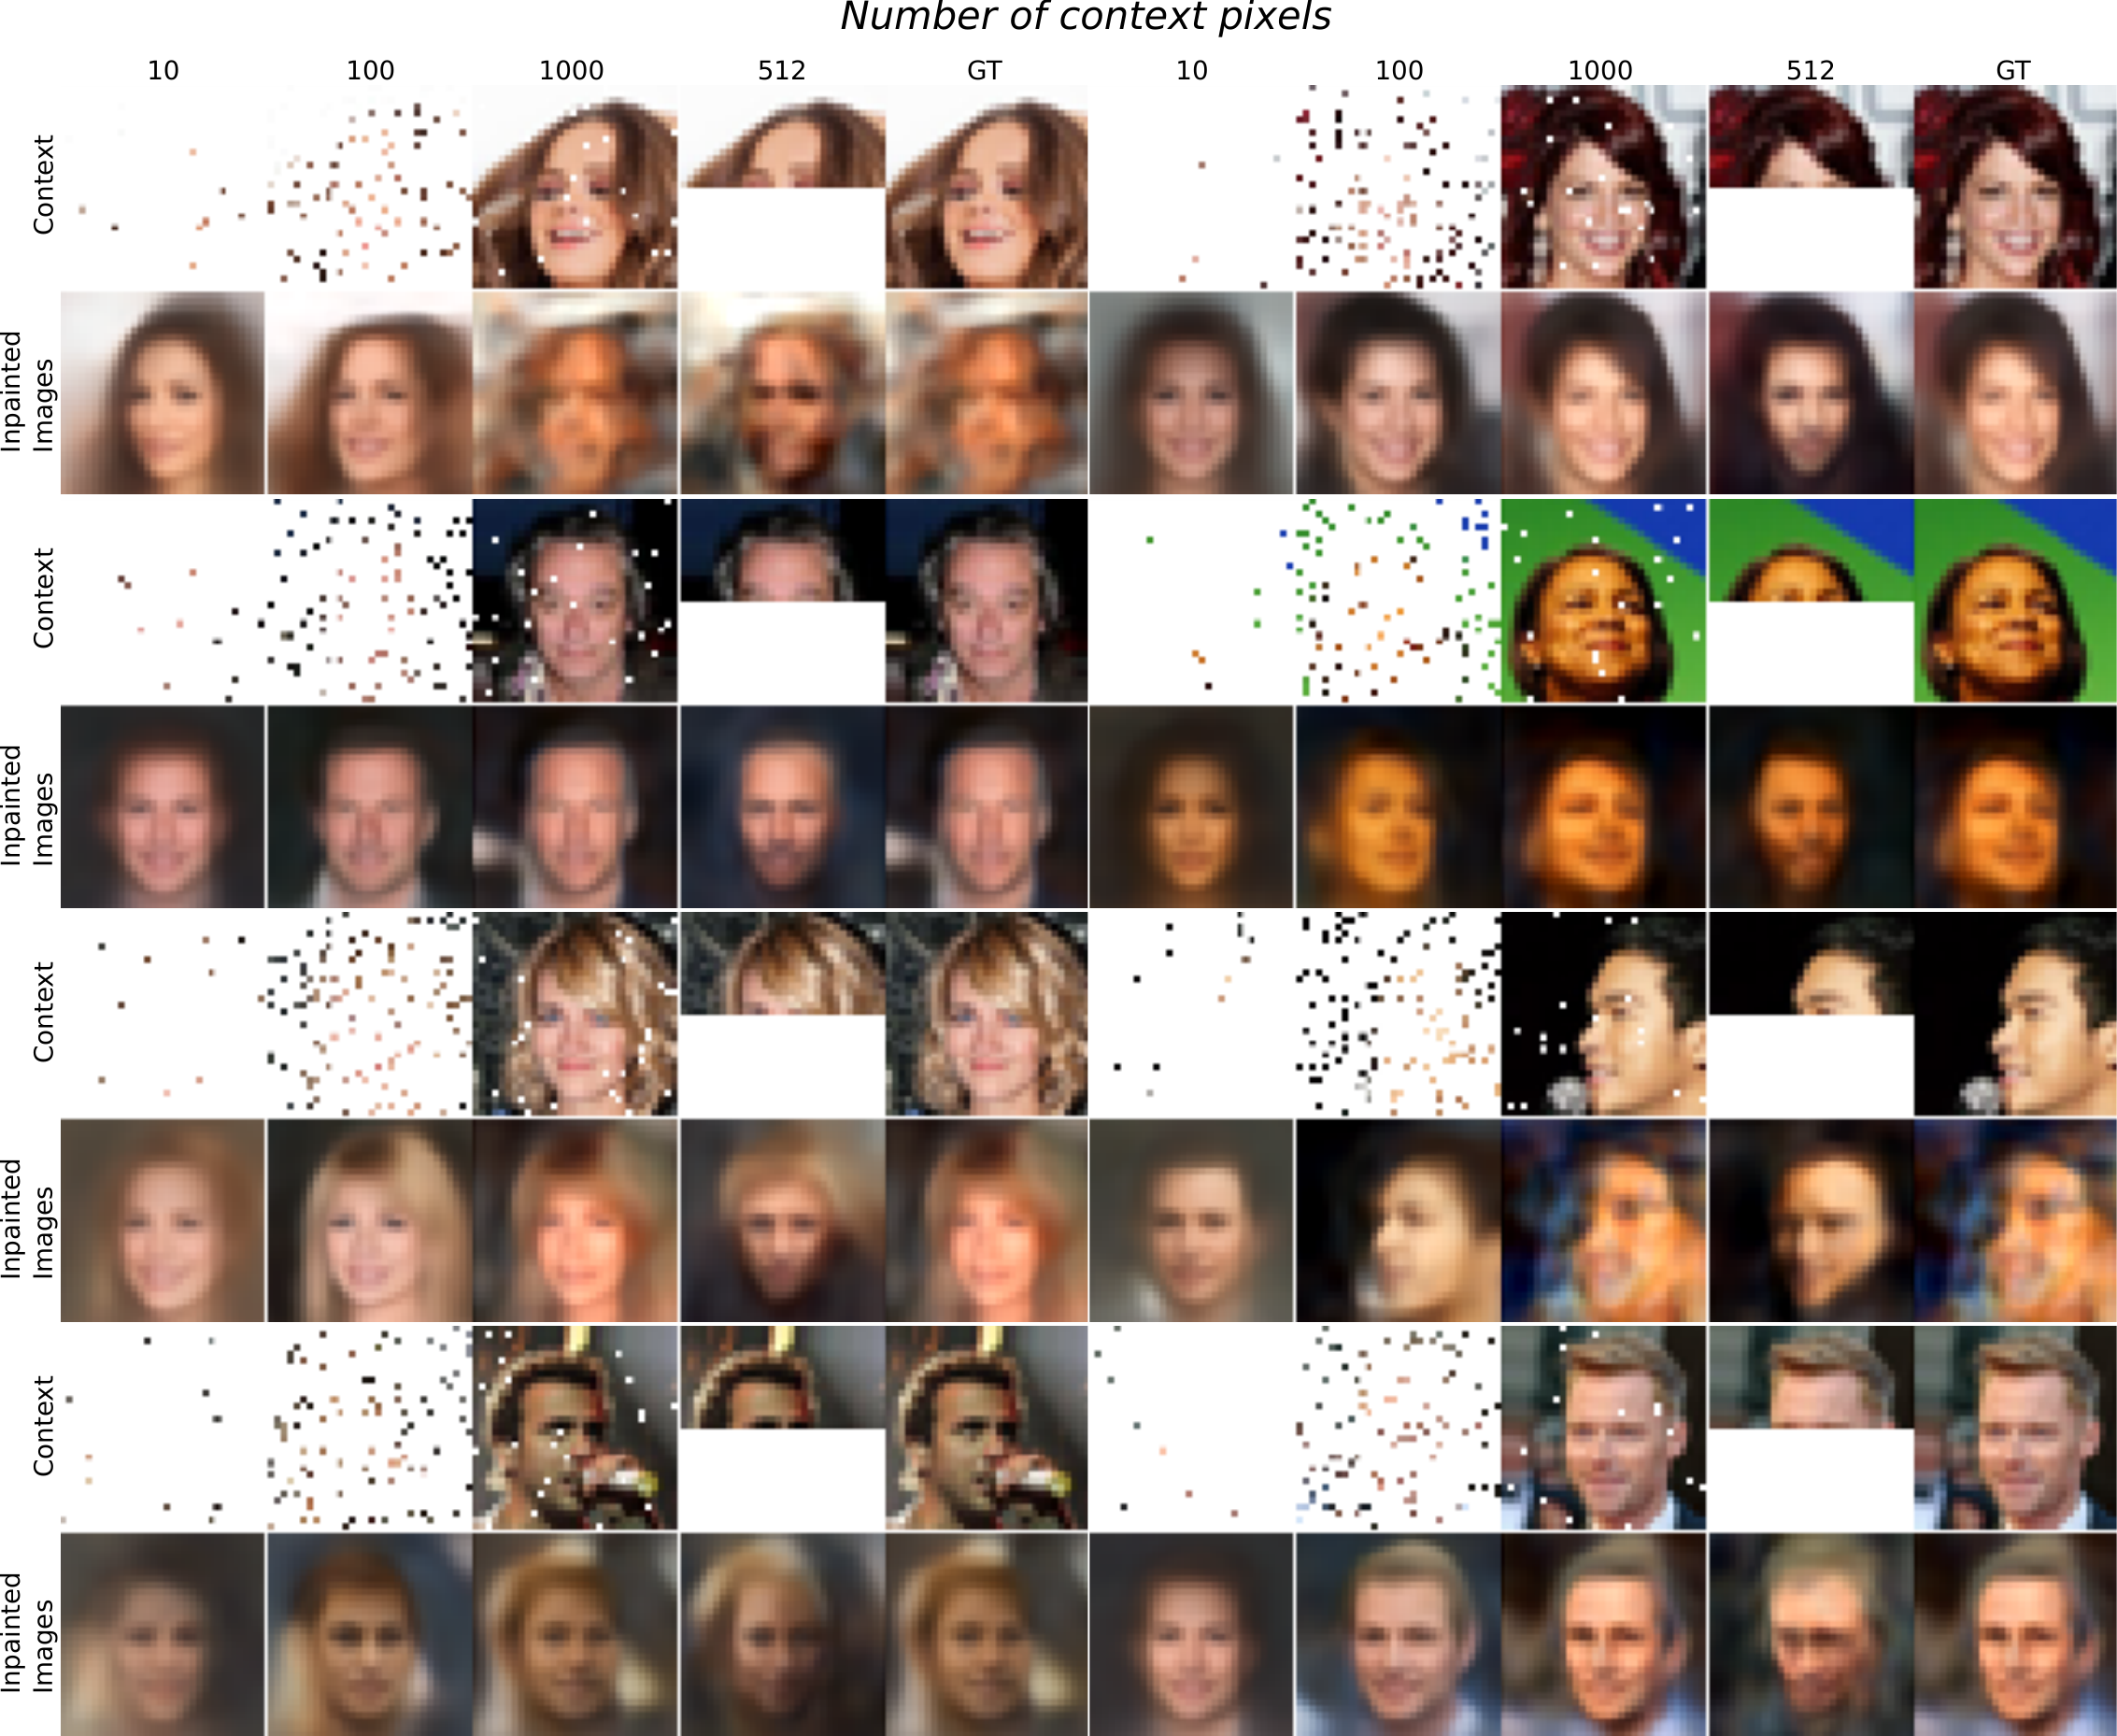} 
	\caption{Additional results using a CNN with partial convolution encoder with a hypernetwork decoder.}
	\label{fig:generalization_partial_conv}
\end{figure}

\begin{table}
	\vspace{-.3cm}
	\caption{Quantitative comparison of inpainting on the CelebA test dataset. Metrics are reported in pixel-wise mean squared error for varying numbers of context pixels. All of the methods for generalizing over \sinet{}s use a hypernetwork as a decoder from latent code to \sinet{} weights. CNP does not report quantitative metrics on half or full images given as context.}
	\label{tab:generalization_additional}
	\centering
	\begin{tabular}{lccccc}
		\toprule
		Number of Context Pixels & 10 & 100 & 1000 & 512 (Half) & 1024 \\
		\midrule
		CNP~\cite{garnelo2018conditional} & 0.039 & 0.016 & 0.009 & - & - \\
		Sine Set Encoder + Hypernet. & 0.035 & 0.013 & 0.009 & 0.022 & 0.009\\
		ReLU Set Encoder + Hypernet. & 0.040 & 0.018 & 0.012 & 0.026 & 0.012\\
		PConv CNN Encoder + Hypernet. & 0.046 & 0.020 & 0.018 & 0.060 & 0.019\\
		CNN Encoder + Hypernet. & \textbf{0.033} & \textbf{0.009} & \textbf{0.008} & \textbf{0.020} & \textbf{0.008} \\
		\bottomrule
	\end{tabular}
\end{table}
