# Supplementary material for: Implicit Neural Representations with Periodic Activation Functions
Source: arXiv:2006.09661 source file (2020-06-17)
Supplement: Supplementary file 6 [file supplement_initialization.tex]

\subsection{Informal statement}
\label{subsec:informal_statement}
\newtheorem{definition}{Definition}[section]
\newtheorem{theorem}{Theorem}[section]
\newtheorem{lemma}[theorem]{Lemma}
Initialization schemes have been shown to be crucial in the training procedure of deep neural networks~\cite{he2015delving,glorot2010understanding}.
%
%Similarly, we empirically observed that bad initializations caused \sinet{} to converge much more slowly.
%%
Here, we propose an initialization scheme for \sinet{} that preserves the distribution of activations through its layers and thus allows us to build deep architectures.
\paragraph{Statement of the initialization scheme.}
We propose to draw weights according to a uniform distribution $W\sim \mathcal{U}(-\sqrt{6/\text{fan\_in}}, \sqrt{6/\text{fan\_in}})$.
We claim that this leads to the input of each sine activation being Gauss-Normal distributed, and the output of each sine activation approximately arcsine-distributed with a standard deviation of $0.5$.
Further, we claim that the form as well as the moments of these distributions do not change as the depth of the network grows.
\newcommand{\reflemma}[1]{\textbf{Lemma~\ref{#1}}}
\paragraph{Overview of the proof.} Our initialization scheme relies on the fact that if the input to a neuron in a layer is distributed the same way as its output, then by a simple recursive argument we can see that the distributions will be preserved throughout the network.

Hence, we consider an input in the interval $[-1,1]$. We assume it is drawn uniformly at random, since we interpret it as a ``normalized coordinate" in our applications. 
We first show in \reflemma{lemma:uni_to_arcsin_dist}, that pushing this input through a sine nonlinearity yields an arcsine distribution. 
The second layer (and, as we will show, all following layers), computes a linear combination of such arcsine distributed outputs (of known variance, \reflemma{lemma:var_arcsin}).
Following Lindeberg's condition for the central limit theorem, this linear combination will be normal distributed \reflemma{lemma:clt_lindenberg}, with a variance that can be calculated using the variance of the product of random variables (\reflemma{lemma:var_prod_rv}).
%, assuming the weights are drawn at random from a uniform distribution with a known variance \reflemma{lemma:var_uni}.
It remains to show that pushing a Gaussian distribution through the sine nonlinearity again yields an arcsine distributed output \reflemma{lemma:gauss_to_arcsin_dist}, and thereby, we may apply the same argument to the distributions of activations of the following layers.

We formally present the lemmas and their proof in the next section before formally stating the initialization scheme and proving it in Section~\ref{subsec:formal_statement_proof_init}. We show empirically that the theory predicts very well the behaviour of the initialization scheme in Section~\ref{subsec:empirical_evaluation}.

\subsection{Preliminary results}
\label{subsec:preliminary_results}
\newcommand{\asindist}[2]{\mathrm{Arcsin}(#1,#2)}
\newcommand{\cdf}[1]{F_{#1}}
\newcommand{\pdf}[1]{f_{#1}}%
\newcommand{\prob}[1]{\mathbb{P}(#1)}
First let us note that the sine function is periodic, of period $2\pi$ and odd: $\sin(-x)=-\sin(x)$, i.e. it is symmetric with respect to the origin. Since we are interested in mapping ``coordinates'' through \sinet, we will consider an input as a random variable $X$ uniformly distributed in [-1,1]. We will thus study, without loss of generality, the frequency scaled \sinet{} that uses the activation
$\sin(\frac{\pi}{2} x)$. Which is half a period (note that the distribution does not change on a full period, it is ``just'' considering twice the half period).
\begin{definition}
The arcsine distribution is defined for a random variable $X$ by its cumulative distribution function (CDF) $\cdf{X}$ such as
\begin{equation}
X\sim\asindist{a}{b}, \text{with CDF: } \cdf{X}(x)=\frac{2}{\pi}\arcsin(\sqrt{\frac{x-a}{b-a}}), \text{with } b>a.\nonumber
\end{equation}
\end{definition}
\begin{lemma}
Given $X\sim\mathcal{U}(-1,1)$, and $Y=\sin(\frac{\pi}{2}X)$ we have $Y\sim\asindist{-1}{1}$.
\label{lemma:uni_to_arcsin_dist}
\end{lemma}
\begin{proof}
The cumulative distribution function (CDF) $\cdf{X}(x)=\prob{X\leq x}$ is defined, for a random variable that admits a continuous probability density function (PDF), $f$ as the integral $\cdf{X}(x) = \int_{-\infty}^{x}f(t)\,dt \label{eq:define_cdf}$.
Hence, for the uniform distribution $\mathcal{U}(-1,1)$ which is $f(x)=\frac{1}{2}$ over the interval $[-1,1]$ and $0$ everywhere else, it is easy to show that:
$\cdf{X}(x) = \frac{1}{2}x + \frac{1}{2}$.

We are interested in the distribution of the output $Y=\sin(\frac{\pi}{2} X)$. Noting that $\sin(\frac{\pi}{2})$ is bijective on $[-1,1]$, we have
\begin{equation}
\cdf{Y}(y) = \prob{\sin(\frac{\pi}{2} X)\leq y} 
= \prob{X \leq \frac{2}{\pi}\arcsin{y}} 
= \cdf{X}(\frac{2}{\pi}\arcsin{y}), \nonumber
\end{equation}
Substituting the CDF $\cdf{X}$, noting it is the uniform distribution which has a compact support (this is [-1,1]), we have
\begin{equation}
\cdf{Y}(y) = \frac{1}{\pi}\arcsin{y} + \frac{1}{2}. \nonumber
\end{equation}
Using the identity $\arcsin\sqrt{x}=\frac{1}{2}\arcsin(2x-1)+\frac{\pi}{4}$, we conclude:
\begin{equation}
	\cdf{Y}(y) \sim \asindist{-1}{1}. \nonumber
\end{equation}
\newcommand{\der}[2]{\frac{d#1}{d#2}}
The PDF can be found, deriving the cdf: 
$
\pdf{Y}(y) = \der{}{y} \cdf{Y}(y) = \frac{1}{\pi} \frac{1}{\sqrt{1-y^2}}.
$
\end{proof}
\newcommand{\variance}[1]{\mathrm{Var}[#1]}
\newcommand{\expec}[1]{\mathrm{E}[#1]}
\begin{lemma}
The variance of $mX+n$ with X a random variable and $m\in\mathbb{R}^+_{\slash 0},n\in\mathbb{R}$ is $\variance{mX+n}=m^2\variance{X}$.
\label{lemma:var_k_arcsin}
\end{lemma}
\begin{proof}
For any random variable with a continuous pdf $\pdf{X}$, its expectation is defined as $\expec{X}=\int_{-\infty}^{\infty}\pdf{X}(x)dx$. The variance is defined as $\variance{X}=\expec{(X-\expec{X})^2}=\expec{X^2}-\expec{X}^2$. Thus, we have $\variance{mX+n}=\expec{(mX+n)^2}-\expec{mX+n}^2=\expec{m^2X^2+2mnX+n^2}-(m\expec{X}+n)^2=m^2(\expec{X^2}-\expec{X}^2)=m^2\variance{X}$.
\end{proof}
\begin{lemma}
The variance of $X\sim\asindist{a}{b}$ is $\variance{X}=\frac{1}{8}(b-a)^2$.
\label{lemma:var_arcsin}
\end{lemma}
\begin{proof}
	First we prove that if $Z\sim\asindist{0}{1}$ then $\variance{Z}=\frac{1}{8}$. We have $\expec{Z}=\frac{1}{2}$ by symmetry, and $\variance{Z}=\expec{Z^2}-\expec{Z}^2=\expec{Z^2}-\frac{1}{4}$. Remains to compute:
\begin{equation}
 \expec{Z^2}= \int_0^1 z^2\cdot \frac{1}{\pi\sqrt{z(1-z)}} \,dz 
 			= \frac{2}{\pi} \int_0^1 \frac{t^4}{ \sqrt{1-t^2}} \,dt
 			= \frac{2}{\pi} \int_0^{\pi/2} \sin^4{u} \,du
 			= \frac{3}{8}, \nonumber
\end{equation}
using a first change of variable: $z=t^2,\, dz=2t\,dt$ and then a second change of variable $t=\sin(u), dt=\cos(u)du$. The integral of $\sin^4(u)$ is calculated remarking it is $(sin^2(u))^2$, and using the formulas of the double angle: $\cos(2u)=2\cos^2(u)-1=1-2\sin^2(u)$.
	
	Second, we prove that if $X\sim\asindist{\alpha}{\beta}$ then the linear combination $mX+n\sim\asindist{\alpha m+n}{\beta m+n}$ with $m\in\mathbb{R}_{\slash0},n\in\mathbb{R}$, (using the same method as in \reflemma{lemma:uni_to_arcsin_dist} with $Y=mX+n$). 
	
	Posing $X=mZ+n$ and using $n=a$ and $m=b-a$, we have $X\sim\asindist{m\cdot0 + n}{m\cdot 1 + n}=\asindist{a}{b}$. Finally, $\variance{X}=\variance{m\cdot Z + n} = m^2\cdot\variance{Z} = (b-a)^2\cdot\frac{1}{8}$ (\reflemma{lemma:var_k_arcsin}).
\end{proof}
\begin{lemma}
For two independent random variables X and Y
\label{lemma:var_prod_rv}
\begin{equation}
	\variance{X\cdot Y} = \variance{X}\cdot\variance{Y} + \expec{Y}^2\cdot\variance{X} + \expec{X}^2\cdot\variance{Y}. \nonumber
\end{equation}
\end{lemma}
\begin{proof}
	See \cite{goodman1960exact}.
\end{proof}
\begin{theorem}
Central Limit Theorem with Lindeberg's sufficient condition. Let $X_k$, $k\in\mathbb{N}$ be independent random variables with expected values $\expec{X_k}=\mu_k$ and variances $\variance{X_k}=\sigma_k$. Posing $s_n^2 = \sum_{k=1}^n \sigma_k^2$. If the $X_k$ statisfy the Lindenberg condition:
\begin{equation}
	\lim_{n\rightarrow\infty} \frac{1}{s_n^2}\sum_{k=1}^{n} \expec{(X_k-\mu_k)^2\cdot\mathbf{1}(|X_k-\mu_k|>\epsilon s_n)} = 0
\end{equation}
$\forall \epsilon>0$, then the Central Limit Theorem (CLT) holds. That is,
\begin{equation}
	S_n = \frac{1}{s_n}\sum_{k=1}^n (X_k-\mu_k),
\end{equation}
converges in distribution to the standard normal distribution as $n\rightarrow\infty$.
\label{lemma:clt_lindenberg}
\end{theorem}
\begin{proof}
	See \cite{lindeberg1922neue,ash2000probability}.
\end{proof}
\begin{figure}[t!]
	\includegraphics[width=\textwidth]{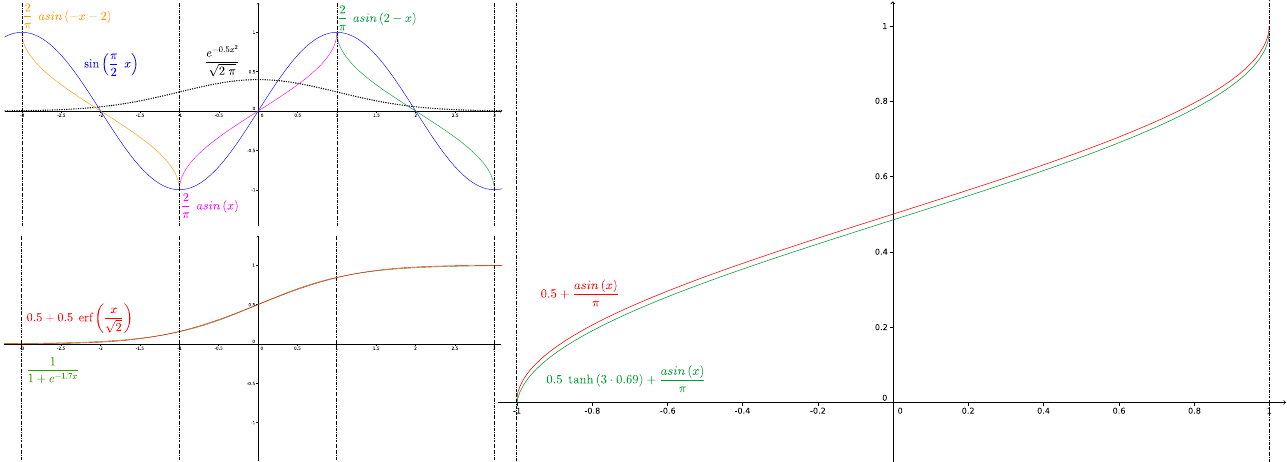}
	\caption{\textbf{Top left:} A plot of the standard normal distribution on $[-3,3]$ as well as the graph of $y=\sin{\frac{\pi}{2}x}$ and its three reciprocal bijections $y=\frac{2}{\pi}\arcsin(-x-2)$, $y=\frac{2}{\pi}\arcsin{x}$ and $y=\frac{2}{\pi}\arcsin(2-x)$ covering the interval $[-3,3]$ in which $99.7\%$ of the probability mass of the standard normal distribution lies. 
	\textbf{Bottom left:} Plot of the approximation of the CDF of the standard normal with a logistic function.
	\textbf{Right:} Comparison of the theoretically derived CDF of the output of a sine nonlinearity (green) and the ground-truth Arcsine CDF (red), demonstrating that a standard normal distributed input fed to a sine indeed yields an approximately Arcsine distributed output.}
	\label{fig:gauss_to_arcsine}
\end{figure}
\begin{lemma}
Given a Gaussian distributed random variable $X\sim\mathcal{N}(0,1)$ and $Y=\sin{\frac{\pi}{2}X}$ we have $Y\sim\asindist{-1}{1}$.
\label{lemma:gauss_to_arcsin_dist}
\end{lemma}
\begin{proof}
For a random variable $X$ normally distributed we can approximate the CDF of its normal distribution with the logistic function, as in \cite{bowling2009logistic}:
\begin{align}
	\cdf{X}(x) &= \frac{1}{2}+\frac{1}{2}\mathrm{erf}(\frac{x}{\sqrt{2}}) \nonumber \\
			   &\approx \big(1+\exp(-\alpha\cdot x)\big)^{-1}  \nonumber\\
			   &\approx \frac{1}{2} + \frac{1}{2}\tanh(\beta\cdot x), \nonumber \label{eq:approx_norm_cdf}
\end{align}
with $\alpha=1.702$ and $\beta=0.690$. Similar to the proof of Lemma~\eqref{lemma:uni_to_arcsin_dist}, we are looking for the CDF of the random variable $Y\sim\sin(\frac{\pi}{2}X)$.
However, the normal distribution does not have compact support.
This infinite support yields an infinite series describing the CDF of Y.

Hence, we make a second approximation that consists in approximating the CDF of Y on the interval $[-3,3]$. Because $X\sim\mathcal{N}(0,1)$, we know that $99.7\%$ of the probability mass of $X$ lies on the compact set $[-3,3]$. Thus, ignoring the other contributions, we have:
\begin{align}
	\cdf{Y}(y) &= \prob{\sin(\frac{\pi}{2} X)\leq y} \nonumber \\
			   &= \cdf{X}(3) - \cdf{X}\big(2-\frac{2}{\pi}\arcsin{x}\big) + \cdf{X}\big(\frac{2}{\pi}\arcsin{x}\big) - \cdf{X}\big(-\frac{2}{\pi}\arcsin{x}-2\big).  \nonumber
\end{align}
Using the logistic approximation of the CDF of $X$, this is:
\begin{align}
	\cdf{X}(x) &= \frac{1}{2}\tanh(3\beta)  \nonumber \\
			   &+ \frac{1}{2} \Big( \tanh(\frac{2\beta}{\pi}z)
				  -\tanh(2\beta(1-\frac{1}{\pi}z))
				  -\tanh(-2\beta(1+\frac{1}{\pi}z))\Big),  \nonumber
\end{align}
with $z=\arcsin{x}$. Using a taylor expansion in $z=0$ (and noting that $\arcsin{0}=0$) we have:
\begin{equation}
	\cdf{X}(x) \overset{0}{=} \frac{1}{2}\tanh(3\beta) + \frac{1}{\pi}\cdot \arcsin{x},  \nonumber
\end{equation}
which approximates $X\sim\asindist{-1}{1}$. Figure~\ref{fig:gauss_to_arcsine} illustrates the different steps of the proofs and the approximations we made.
\end{proof}
\begin{lemma}
	The variance of $X\sim\mathcal{U}(-a,b)$ is $\variance{X}=\frac{1}{12}(b-a)^2$
	\label{lemma:var_uni}
\end{lemma}
\begin{proof}
	$\expec{X}=\frac{a+b}{2}$. $\variance{X}=\expec{X^2}-\expec{X}^2=\frac{1}{b-a}[\frac{x^3}{3}]_a^b - (\frac{a+b}{2})^2=\frac{1}{b-a}\frac{b^3-a^3}{3}-(\frac{a+b}{2})^2$, developing the cube as $b^3-a^3=(b-a)(a^2+ab+b^2)$ and simplifying yields the result.
\end{proof}
\subsection{Formal statement and proof of the initialization scheme}
\label{subsec:formal_statement_proof_init}
\begin{theorem}
For a uniform input in $[-1,1]$, the activations throughout a \sinet{} are standard normal distributed before each sine nonlinearity and arcsine-distributed after each sine nonlinearity, irrespective of the depth of the network, if the weights are distributed uniformly in the interval $[-c,c]$ with $c=\sqrt{6/\text{fan\_in}}$ in each layer.
\begin{proof}
Assembling all the lemma, a sketch of the proof is:
\setlist{leftmargin=2.5mm}
\begin{itemize}
	\item Each output $X_l$ for the layer $l$ is $X_l\sim\asindist{-1}{1}$ (first layer: from a uniform distribution \reflemma{lemma:uni_to_arcsin_dist}, next layers: from a standard-normal \reflemma{lemma:gauss_to_arcsin_dist}) and $\variance{X_l}=\frac{1}{2}$ (\reflemma{lemma:var_arcsin}).
	\item The input to the layer $l+1$ is $w_l^T X_l=\sum_i^n w_{i,l} X_{i,l}$ (bias does not change distribution for high enough frequency). Using weights $w_i^l\sim\mathcal{U}(-c,c)$ we have $\variance{w_l^T X_l} = \variance{w_l}\cdot\variance{X_l}=\frac{1}{12}(2c)^2\cdot\frac{1}{2}=\frac{1}{6}c^2$ (from the variance of a uniform distribution \reflemma{lemma:var_uni}, and an arcsine distribution \reflemma{lemma:var_arcsin}, as well as their product \reflemma{lemma:var_prod_rv}).
	\item Choosing $c=\sqrt{\frac{6}{n}}$, with the fan-in $n$ (see dot product above) and using the CLT with weak Lindenberg's condition we have $\variance{w_l^T X_l}=n\cdot\frac{1}{6}\frac{6}{n}=1$ \reflemma{lemma:clt_lindenberg} and $w_l^T X_l \sim\mathcal{N}(0,1)$
	\item This holds true for all layers, since normal distribution through the sine non-linearity yields again the arcsine distribution \reflemma{lemma:var_k_arcsin}, \reflemma{lemma:gauss_to_arcsin_dist}
\end{itemize}
\end{proof}
\end{theorem}

\subsection{Empirical evaluation}
\label{subsec:empirical_evaluation}
We validate our theoretical derivation with an experiment.
We assemble a 6-layer, single-input \sinet{} with 2048 hidden units, and initialize it according to the proposed initialization scheme.
We draw $2^8$ inputs in a linear range from $-1$ to $1$ and plot the histogram of activations after each linear layer and after each sine activation.
We further compute the 1D Fast Fourier Transform of all activations in a layer.
Lastly, we compute the sum of activations in the final layer and compute the gradient of this sum w.r.t. each activation.
The results can be visualized in Figure~\ref{fig:activation_statistics}. 
The distribution of activations nearly perfectly matches the predicted Gauss-Normal distribution after each linear layer and the arcsine distribution after each sine nonlinearity.
As discussed in the main text, frequency components of the spectrum similarly remain comparable, with the maximum frequency growing only slowly.
We verified this initialization scheme empirically for a 50-layer \sinet{} with similar results.
Finally, similar to the distribution of activations, we plot the distribution of gradients and empirically demonstrate that it stays almost perfectly constant across layers, demonstrating that \sinet{} does not suffer from either vanishing or exploding gradients at initialization.
We leave a formal investigation of the distribution of gradients to future work.

\subsection{About $\omega_0$}
As discussed above, we aim to provide each sine nonlinearity with activations that are standard normal distributed, except in the case of the first layer, where we introduced a factor $\omega_0$ that increased the spatial frequency of the first layer to better match the frequency spectrum of the signal.
However, we found that the training of \sinet{} can be accelerated by leveraging a factor $\omega_0$ in \emph{all} layers of the \sinet{}, by factorizing the weight matrix $\mathbf{W}$ as $\mathbf{W} = \hat{\mathbf{W}} * \omega_0$, choosing $\hat{W} \sim \mathcal{U}(-\sqrt{\frac{c}{\omega_0^2 n}}, \sqrt{\frac{c}{\omega_0^2 n}})$. 
This keeps the distribution of activations constant, but boosts gradients to the weight matrix $\hat{\mathbf{W}}$ by the factor $\omega_0$ while leaving gradients w.r.t. the input of the sine neuron unchanged.

\begin{figure}
	\centering
	\includegraphics[]{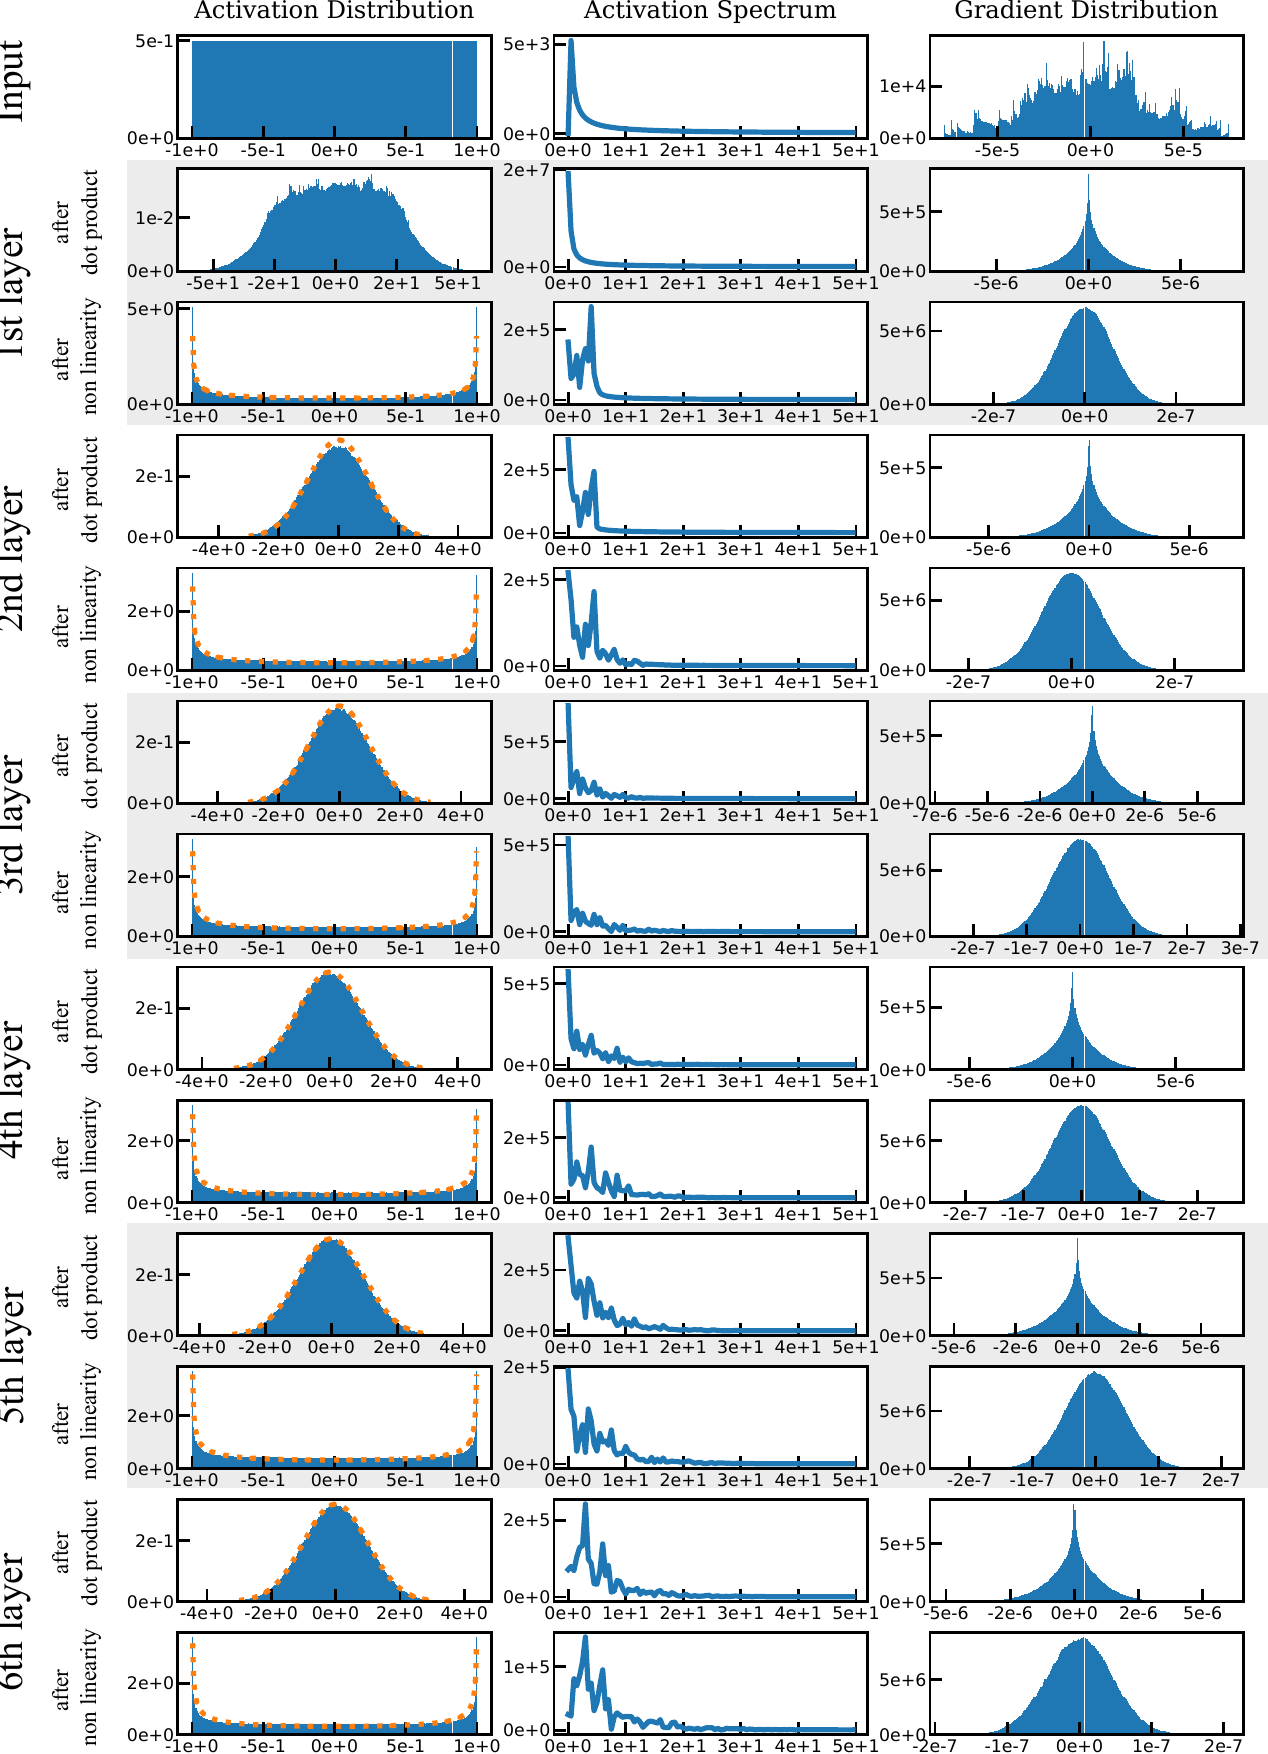}
	\caption{Activation and gradient statistics at initialization for a 6-layer \sinet{}. Increasing layers from top to bottom. Orange dotted line visualizes analytically predicted distributions. Note how the experiment closely matches theory, activation distributions stay consistent from layer to layer, the maximum frequency throughout layers grows only slowly, and gradient statistics similarly stay consistent from layer to layer.}
	\label{fig:activation_statistics}
\end{figure}
