# Supplementary material for: Implicit Neural Representations with Periodic Activation Functions
Source: arXiv:2006.09661 source file (2020-06-17)
Supplement: Supplementary file 7 [file supplement_poisson.tex]

\subsection{Architecture Comparisons}
\begin{figure}
	\includegraphics[width=\textwidth]{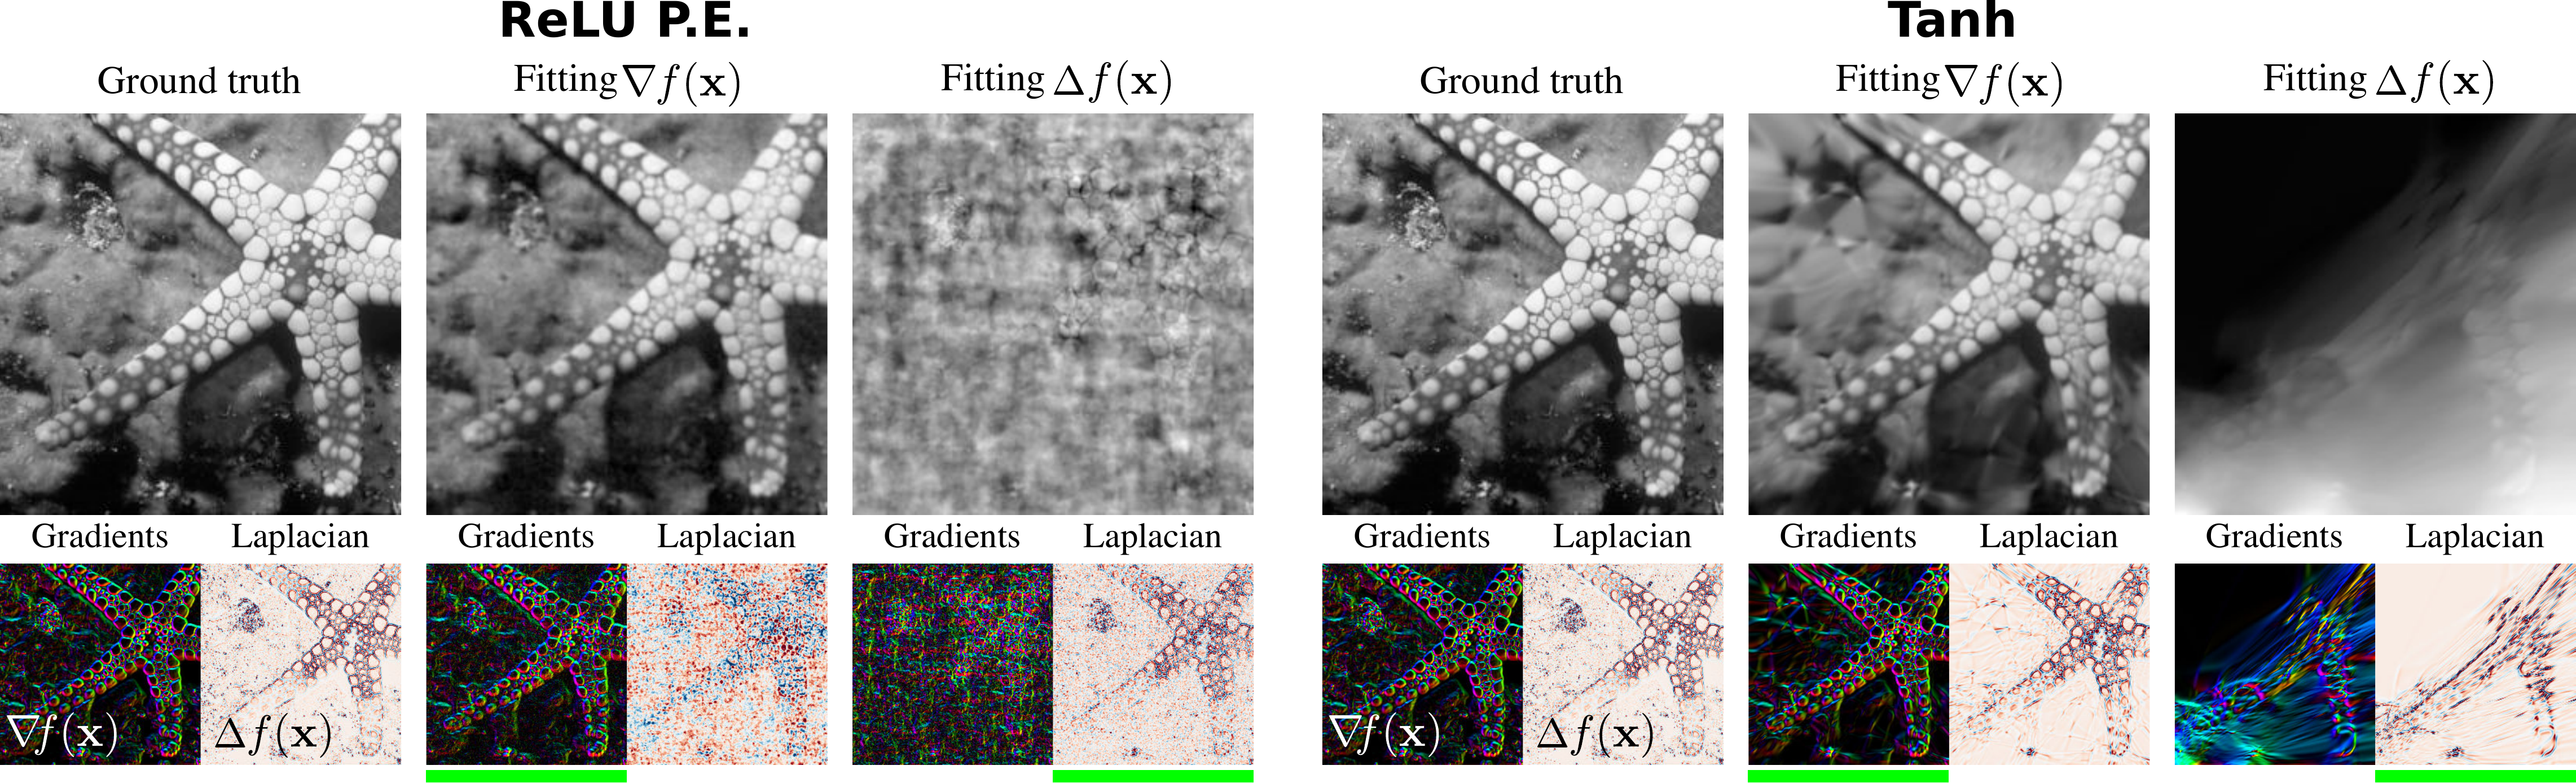} 
	\caption{Poisson image reconstruction using the ReLU P.E. (left) and tanh (right) network architectures. For both architectures, image reconstruction from the gradient is of lower quality than \sinet{}, while reconstruction from the Laplacian is not at all accurate.}
	\label{fig:poisson_PE}
\end{figure}

To show that our representation is unique in being able to represent signals while being supervised solely by their derivatives, we test other neural network architectures and activation functions on the Poisson image reconstruction task. 
We show that the performance of the ReLU P.E. network architecture, which performed best on the single image fitting task besides \sinet{}, is not as accurate in supervising on derivatives. This is shown in Fig.~\ref{fig:poisson_PE}. Additionally, in Tab.~\ref{tab:poisson}, we compare the PSNR of the reconstructed image, gradient image, and Laplace image between various architectures for Poisson image reconstruction.

One interesting observation from Tab.~\ref{tab:poisson} is that other architectures such as ReLU P.E. have trouble fitting the Laplace and gradient images even when directly supervised on them, despite being able to fit images relatively accurately. 
%It is challenging to quantitatively evaluate the higher order derivative fit due to scale ambiguity, and one side effect of computing metrics on the normalized and colorized images is that the ``grainy'' effect (in ReLU P.E. architecture) contributes significantly to the PSNR error. 
This may be because the ground truth gradient and Laplace images have many high frequency features which are challenging to represent with any architecture besides \sinet{}s. In the normalized and colorized images (which PSNR is computed upon), the gradient image fit with ReLU P.E. has ``grainy'' effects which are more noticeable on gradient and Laplacian images than on natural images.

%\begin{table}
	%\vspace{-.3cm}
	%\caption{Quantitative comparison of reconstructed image, gradient image, and Laplace image in the Poisson image reconstruction task on the starfish image. Reconstruction accuracy is reported in PSNR after the images have been colorized and normalized.}
	%\label{tab:poisson}
	%\centering
	%\begin{tabular}{l|cc|cc|cc}
		%\toprule
		%Model \& Supervision$\rightarrow$ & \sinet{} & \sinet{} & ReLU P.E. & ReLU P.E. & Tanh & Tanh \\
 		%Reconstruction$\downarrow$ & Grad. & Laplacian & Grad. & Laplacian & Grad. & Laplacian \\
		%\midrule
		%Image & \textbf{32.91} & \textbf{14.95} & 26.35 & 11.14 & 25.79 & 7.11 \\
		%Grad. & \textbf{46.85} & \textbf{23.45} & 19.33 & 11.35 & 19.11 & 11.14 \\
		%Laplacian & \textbf{19.88} & \textbf{57.13} & 14.24 & 18.31 & 18.59 & 16.35 \\
		%\bottomrule
	%\end{tabular}
%\end{table}

\begin{table}
	\vspace{-.3cm}
	\caption{Quantitative comparison of reconstructed image, gradient image, and Laplace image in the Poisson image reconstruction task on the starfish image. Reconstruction accuracy is reported in PSNR after the images have been colorized and normalized.}
	\label{tab:poisson}
	\centering
	\begin{tabular}{lcccccc}
		\toprule
		Model  & \multicolumn{2}{c}{Tanh} & \multicolumn{2}{c}{ReLU P.E.} & \multicolumn{2}{c}{\sinet{}} \\
 		Supervised on  & Grad. & Laplacian & Grad. & Laplacian & Grad. & Laplacian \\
		\midrule
		Reconstructed Image & 25.79 & 7.11& 26.35 & 11.14  & \textbf{32.91} & \textbf{14.95} \\
		Reconstructed Grad. & 19.11 & 11.14 & 19.33 & 11.35  & \textbf{46.85} & \textbf{23.45} \\
		Reconstructed Laplacian  & 18.59 & 16.35 & 14.24 & 18.31 & \textbf{19.88} & \textbf{57.13} \\
		\bottomrule
	\end{tabular}
\end{table}

\subsection{Implementation \& Reproducibility Details}

\paragraph{Data.} We use the BSDS500~\cite{MartinFTM01}, which we center-crop to $321\times321$ and resize to $256\times256$. The starfish image is the 19th image from this dataset. We will make the bear and pyramid images used in the Poisson image editing experiment publicly available with our code. The ground truth gradient image is computed using the Sobel filter, and is scaled by a constant factor of 10 for training. The ground truth Laplace image is computed using a Laplace filter, and is scaled by a constant factor of 10,000 for training.

\paragraph{Architecture.} We use the same 5-layer \sinet{} MLP for all experiments on fitting images and gradients.

\paragraph{Hyperparameters.} We train for 10,000 iterations, and at each iteration fit on every pixel in the gradient or Laplacian image. We use the Adam optimizer with a learning rate of $1\times 10^{-4}$ for all experiments, including the Poisson image editing experiments.

\paragraph{Runtime.} We train for 10,000 iterations, requiring approximately 90 minutes to fit and evaluate a \sinet{}.

\paragraph{Hardware.} The networks are trained using NVIDIA Quadro RTX 6000 GPUs with 24 GB of memory.
