# Supplementary material for: Implicit Neural Representations with Periodic Activation Functions
Source: arXiv:2006.09661 source file (2020-06-17)
Supplement: Supplementary file 8 [file supplement_remarks.tex]

\subsection{About periodicity}
Here, we provide a few remarks on the periodicity of the functions parameterized by \sinet{}.
It is known that the sum of two periodic signals is itself periodic with a period that is equal to the least common multiple of the periods of the two summands, if and only if the two periods are rational multiples of each other~\cite{olmsted1959real}. If the ratio of the two periods is irrational, then their sum will \emph{not} be periodic itself.
Due to the floating-point representation in neural network libraries, this case cannot occur in practice --- we thus conclude that all functions parameterized by \sinet{} will themselves be periodic.
Yet, the period of the resulting function may in practice be several orders of magnitudes larger than the period of each \sinet{} neuron. Indeed, when sampling a \sinet{} outside its input range, we did not find repetitions of the signal, but essentially noise.
\subsection{About $\omega_0$}
As discussed in the initialization section, we aim to provide each sine nonlinearity with activations that are standard normal distributed, except in the case of the first layer, where we introduced a factor $\omega_0$ that increased the spatial frequency of the first layer to better match the frequency spectrum of the signal.
However, we found that the training of \sinet{} can be accelerated by leveraging a factor $\omega_0$ in \emph{all} layers of the \sinet{}, by factorizing the weight matrix $\mathbf{W}$ as $\mathbf{W} = \hat{\mathbf{W}} * \omega_0$, choosing $\hat{W} \sim \mathcal{U}(-\sqrt{\frac{c}{\omega_0^2 n}}, \sqrt{\frac{c}{\omega_0^2 n}})$. 
This keeps the distribution of activations constant, but boosts gradients to the weight matrix $\mathbf{W}$ by the factor $\omega_0$ while leaving gradients w.r.t. the input of the sine neuron unchanged.
%
%, as can be seen by taking the partial derivatives of a single sine neuron $\mathbf{y}$:
%%
%\begin{align}
%\pdv{\mathbf{y}}{\hat{\mathbf{W}}} &=\pdv{}{\hat{\mathbf{W}}} \sin(\omega_0 \hat{\mathbf{W}} \mathbf{x} + \mathbf{b}) = \omega_0 \mathbf{x} \mathcal{I} \cos(\omega_0 \hat{\mathbf{W}} \mathbf{x} + \mathbf{b}) \\	\pdv{\mathbf{y}}{\mathbf{x}} &= \pdv{}{\mathbf{x}} \sin(\omega_0 \hat{\mathbf{W}} \mathbf{x} + \mathbf{b}) = \omega_0 \hat{\mathbf{W}}^T \cos(\omega_0 \hat{\mathbf{W}} \mathbf{x} + \mathbf{b})	
%\end{align}
%%
%with the identity matrix $\mathcal{I}$.
%%
%Thus, gradients for $\hat{\mathbf{W}}$ are boosted by a factor of $\omega_0$, while the distribution of gradients w.r.t. $\mathbf{x}$ remains the same, as $\mathbf{W}^T=\omega_0 \hat{\mathbf{W}}^T \sim \mathcal{U}(-\sqrt{\frac{c}{n}}, \sqrt{\frac{c}{n}})$. In practice, we choose $\omega_0=30$.
