# Supplementary material for: Implicit Neural Representations with Periodic Activation Functions
Source: arXiv:2006.09661 source file (2020-06-17)
Supplement: Supplementary file 9 [file supplement_sdf.tex]

We performed an additional baseline using the ReLU positional encoding \cite{mildenhall2020nerf} shown in Figure~\ref{fig:relu_pe}. Similar to the results we obtained using the ReLU positional encoding on images, zero-level set of the SDF, in which the shape is encoded features high-frequencies that are not present while the level of details remains low (despite being much higher that in ReLU, see main paper).

\paragraph{Data.} We use the Thai statue from the The Stanford 3D Scanning Repository (http://graphics.stanford.edu/data/3Dscanrep/). The room is a Free 3D model from Turbosquid.com. We sample each mesh by subdividing it until we obtain 10 million points and their normals. Those are then converted in .xyz formats we load from our code. 

\paragraph{Architecture.} We use the same 5-layer \sinet{} MLP for all experiments on SDF, using 256 units in each layer for the statue and 1024 units in each layer for the room.

\paragraph{Hyperparameters.} We train for 50,000 iterations, and at each iteration fit on every voxel of the volume. We use the Adam optimizer with a learning rate of $1\times 10^{-4}$ for all experiments. We use the cost described in our paper:
\begin{equation}
	%\mathcal{L}_{\mathrm{sdf}} = \int_{\Omega\cup\sdfdomainzero} % the zero-level set is part of the domain, so their union is still the wholedomain	
	\mathcal{L}_{\mathrm{sdf}} \! = \! \lambda_1\int_{\sdfdomain}
	\big\| \left|\grad_\mathbf{x} \implicit(\mathbf{x}) \right| - 1 \big\|
	d \mathbf{x}
	+
	\int_{\sdfdomainzero}
	%\lambda_{\sdfdomainzero}\:
	%\Big( 
	\!\!
		  \lambda_2\left\| \implicit ( \mathbf{x} ) \right\|
	 	+ \lambda_3\big(1 - \langle \grad_\mathbf{x} \implicit(\mathbf{x}), \mathbf{n}(\mathbf{x}) \rangle  \big)
	 %\Big)
	d \mathbf{x}
	+
	\lambda_2\int_{\sdfdomain\setminus\sdfdomainzero} \!\!\!\!
	 % \lambda_{\sdfdomain\setminus\sdfdomainzero}\: \psi\big(u(x)\big)
	\psi \big(\implicit(\mathbf{x})\big)
	d \mathbf{x},
\end{equation}
with the Eikonal constraint (gradient = 1) multiplied by $\lambda_1=5\cdot 10^1$, the signed distance function constraint as well as the off-surface penalization (the regularizer) multiplied by $\lambda_2=3\cdot 10^3$, and the oriented surface/normal constraint multiplied by $\lambda_3=1\cdot 10^2$.
\paragraph{Runtime.} We train for 50,000 iterations, requiring approximately 6h hours to fit and evaluate a \sinet{}. Though, we remark that \sinet{} converge already very well after around 5,000-7,000 iterations, much more iterations are needed for the baselines, hence the number of 50,000 iterations.

\paragraph{Hardware.} The networks are trained using NVIDIA GTX Titan X GPUs with 12 GB of memory.

\begin{figure}[t!]
	\includegraphics[width=\textwidth]{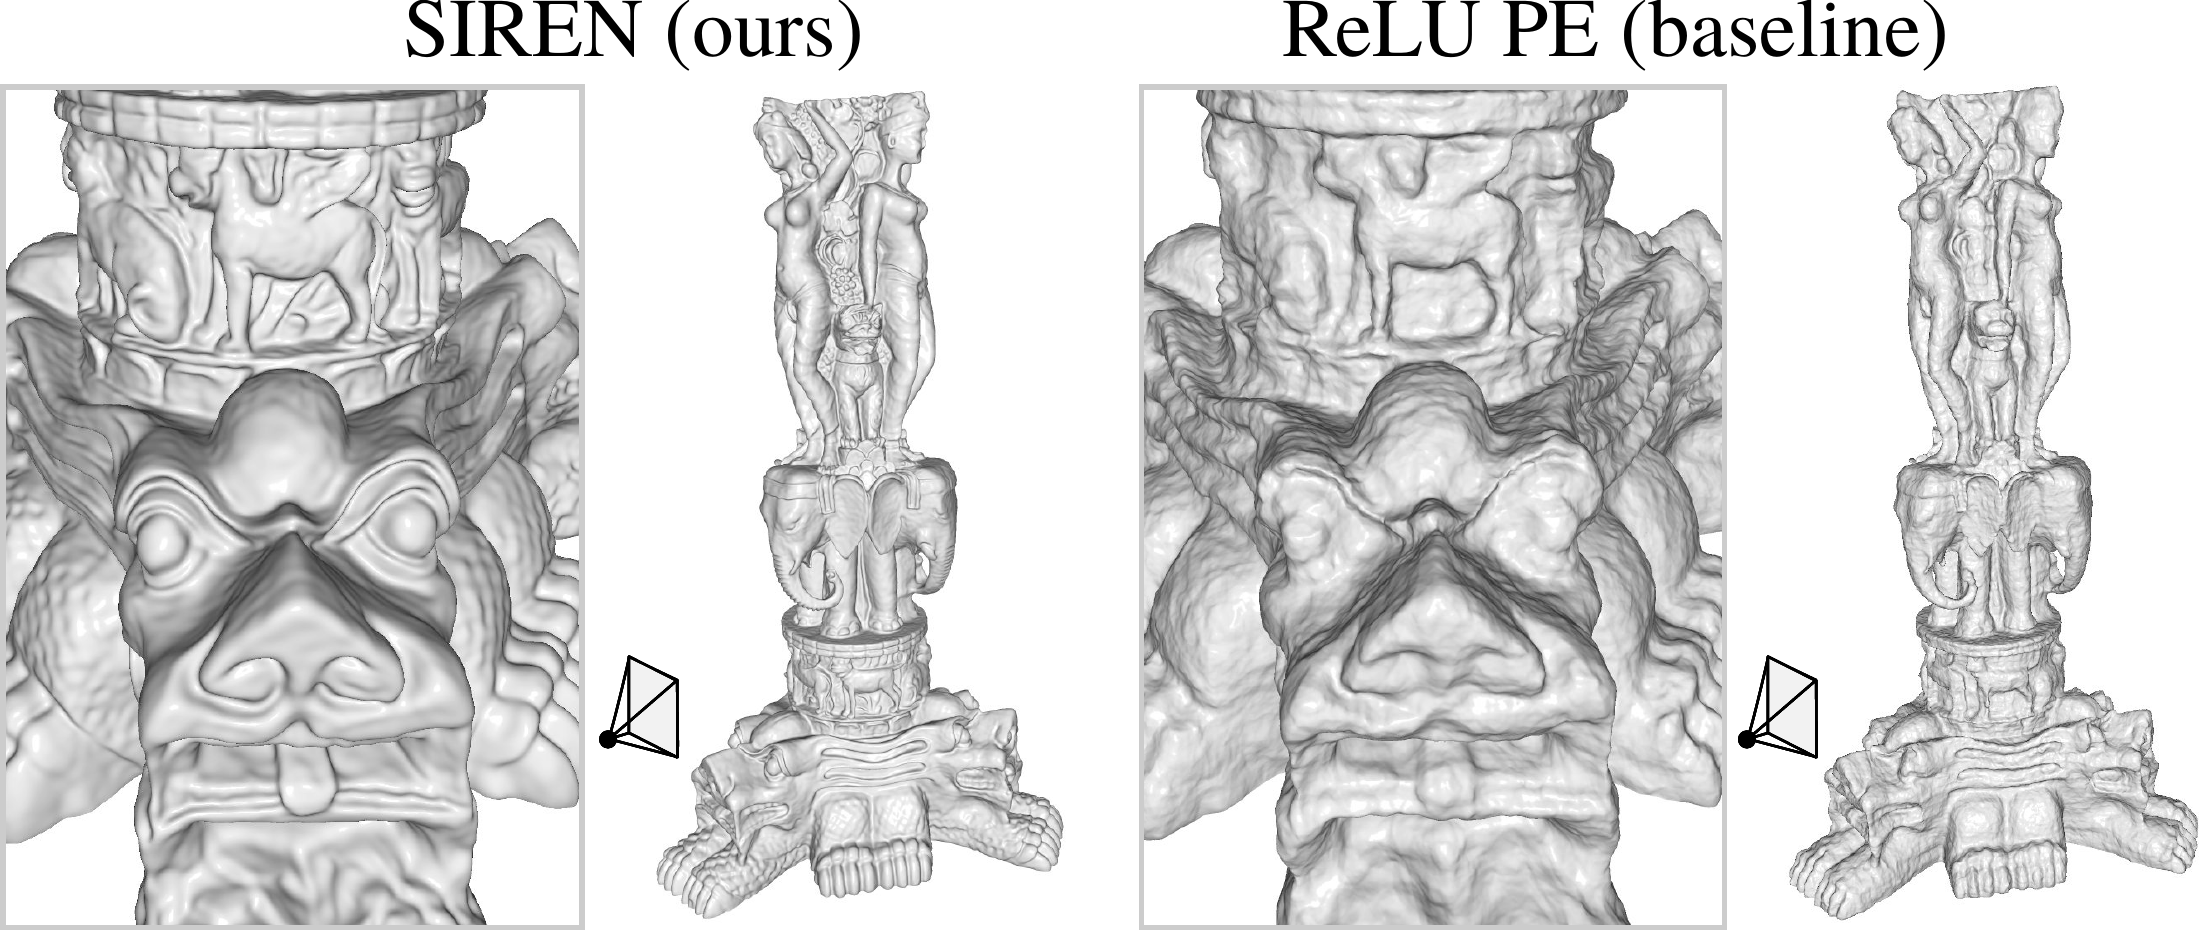}
	\caption{A comparison of \sinet{} used to fit a SDF from an oriented point clouse against the same fitting performed by an MLP using a ReLU PE (proposed in \cite{mildenhall2020nerf}).}
	\label{fig:relu_pe}
\end{figure}
