# Supplementary material for: Implicit Neural Representations with Periodic Activation Functions
Source: arXiv:2006.09661 source file (2020-06-17)
Supplement: Supplementary file 10 [file supplement_video.tex]

\begin{figure}
    \centering
    \includegraphics[]{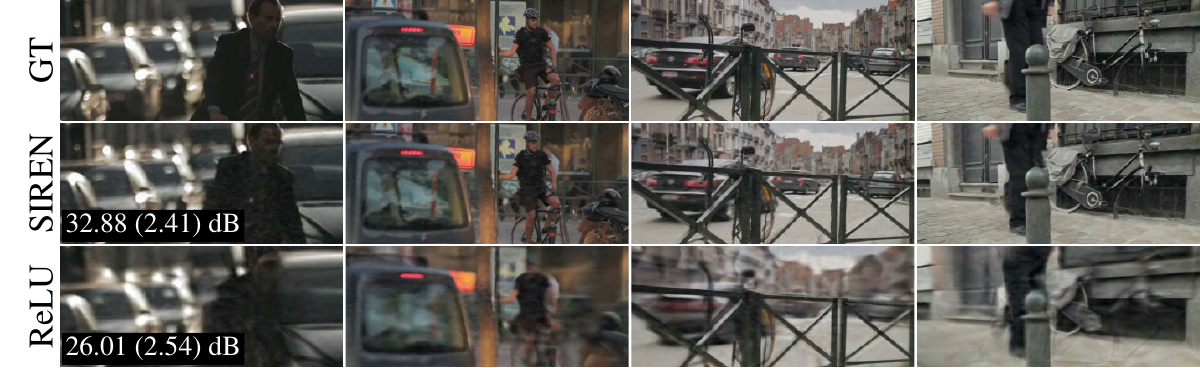}
    \caption{Example frames from fitting a video with \sinet{} and ReLU MLPs. \sinet{} more accurately reconstructs fine details in the video. Mean (and standard deviation) of the PSNR over all frames is reported.}
    \label{fig:bikes_video}
\end{figure}

We fit videos using \sinet{} and a baseline ReLU architecture as described in the main paper and video. We also fit a second video, which consists of various vehicles moving in traffic and outdoor scenes, shown in Fig.~\ref{fig:bikes_video}. Again, \sinet{} shows improved representation of fine details in the scene.  
In the following we provide additional implementation details.

\subsection{Reproducibility \& Implementation Details}
\paragraph{Data.}
The first dataset consists of a video of a cat, which is permissively licensed and available at the time of this writing from \url{https://www.pexels.com/video/the-full-facial-features-of-a-pet-cat-3040808/}. The second dataset is the ``bikes sequence''  available from the scikit-video Python package described here \url{http://www.scikit-video.org/stable/datasets.html}. We crop and downsample the cat video to 300 frames of $512\times 512$ resolution. The second dataset consists of 250 frames fit at the original resolution of $272 \times 640$ pixels.  
\paragraph{Architecture.}
The \sinet{} and ReLU architectures use 5 layers with a hidden layer size of 1024.   

\paragraph{Hyperparameters.}
The Adam optimizer with a learning rate of $1\times 10^{-4}$ was used for all experiments. We set the batch size to fill the memory of the GPUs (roughly 160,000). 

\paragraph{Runtime.}
We train the videos for 100,000 iterations, requiring approximately 15 hours.

\paragraph{Hardware.}
The networks are trained using NVIDIA Titan X (Pascal) GPUs with 12 GB of memory.
